# Supplementary material for: Runtime Verification and Field-based Testing for ROS-based Robotic Systems
Source: arXiv:2404.11498 source file (2024-08-21)
Supplement: Supplementary file 1 [file appendix.tex]

\section*{APPENDIX} \label{sec:appendix}

In the appendix we describe two sets of guidelines: guidelines for enabling and facilitating runtime verification and field-based testing for ROS-based applications through development are presented in ~\cref{sec:facilitate_fulllist} and guidelines for providing quality assurance through runtime verification and field-based testing for ROS-based applications are detailed in ~\cref{sec:test_fulllist}. After the follow-up questionnaire we changed three guidelines CI2, MTA2, PE2, according to the following rule: additions are marked with {\color{blue} blue} highlight and deletions with {\color{red} red}, we also point out the changes with footnote markings.

\section{Guidelines for Development to Support Runtime Verification and Field-Based Testing}\label{sec:facilitate_fulllist}
 
 In this section, we detail eight guidelines for facilitating the verification of ROS-based applications through development activities. Our approach to facilitate verification lies on providing guidance to robotics software developers.
 The group of Constraint Identification (CI) guidelines contains three guidelines, CI1, CI2, and CI3, devoted to identifying constraints of different nature, i.e., timing constraints, security and privacy constraints, and safety constraints. The group of Code Design and Implementation (CD) guidelines contains two guidelines, CD1 recommending to design ROS nodes with single responsibility and CD2 guiding towards ensuring global time monotonicity of events and states. The last group contains four Instrumentation (I) guidelines. I1, I2, and I3 focus on providing APIs for querying and updating an internal lifecycle (I1), for logging and filtering (I2), and for injecting faults in execution scenarios (I3). The last one (I4) focuses on isolating components for testing.

\subsection{CI1. Identify timing constraints}\label{sec:CI1}

\subsubsection{Context (WHEN)} 
Timing constraints, also known as ``deadline'' or ``timing requirements'', define temporal requirements that real-time systems must adhere to~\cite{schutz2007testability}. These constraints can be categorized as soft, firm, or hard, and they play a significant role in determining whether the system respects timing concerns. Since ROS-based systems often involve control nodes (such as attitude control and state estimation~\cite{beul:2017}), which typically have real-time requirements, identifying timing constraints becomes even more critical. %However, a recent study highlights the lack of support for real-time constraints in the software engineering research of ROS-based robotic systems, emphasizing the need for more attention in this domain~\cite{albonico2023software}. 
%Initially conceived as a means to handle difficult or costly-to-reproduce failures, field testing has seen limited studies addressing real-time issues, particularly in the realm of autonomous systems~\cite{bertolino:2021}.

\subsubsection{Reason (WHY)} Identifying timing constraints is crucial for ROS-based systems as these constraints define the system's temporal requirements. However, a recent study highlights the lack of support for real-time constraints in the software engineering research of ROS-based robotic systems, emphasizing the need for more attention in this domain~\cite{albonico2023software}. Initially conceived as a means to handle difficult or costly-to-reproduce failures, field testing has seen limited studies addressing real-time issues, particularly in the realm of autonomous systems~\cite{bertolino:2021}.

\subsubsection{Suggestion (WHAT)} %The development team should identify timing constraints to ensure that no real-time requirements will be neglected during the system testing.
The development team should identify timing constraints to ensure that no real-time requirements will be neglected during the system testing. For instance,  Autoware\_Perf (git: azu-lab/ROS2-E2E-Evaluation) allows for the calculation of response time and latency in  ROS 2 applications; such measurements may be used as hard constraints to testing the system. Also, one may identify real-time constraints with respect to synchronization between robots, sensor data processing time, or fault detection and recovery.

\subsubsection{Process (HOW)} %We divide the activity of identifying timing constraints into understanding which timing constraints may be important in the application domain of the robot and constraints specification. 
Typical timing constraints that cross-cut in robotics domains stand for response time~\cite{chaaban2023new}, latency, synchronization time~\cite{lewis:2022}, fault detection and recovery time, and power management time. The means to specify such constraints vary from informal to formal languages (we invite the interested reader to check guidelines of the group property specification - SDB1 and SDB2. The developers team may use \href{https://github.com/azu-lab/ROS2-E2E-Evaluation}{Autoware\_Perf~\faicon{{github}}}\cite{li2022autoware_perf} to calculate response time and latency, for example.%We indicate formal languages to unambiguously encode the expected robotic behavior in machine-readable formalisms such as TCTL, (DT-)MTL, and STL.

\subsubsection{Exemplars}~\\ 
\textbf{Typical Timing Constraints.} Real-time constraints may be subject to the domain and the objectives of the runtime assessment. We provide a comprehensive list of constraints that may be interesting to address when considering testing ROS-based systems. We use \href{https://github.com/azu-lab/ROS2-E2E-Evaluation}{Autoware\_Perf~\faicon{{github}}}\cite{li2022autoware_perf} to illustrate how to collect response time and latency with practical examples.

\begin{itemize}
    \item \textbf{Response time} is the period a ROS-based system takes to react to one or more stimuli from the environment. Specific to the ROS domain, Chaaban, K. defines response time in ROS 2 as the \textit{``duration from the release instant to the completion of the job execution''}~\cite{chaaban2023new}. To collect callback response time, Autoware\_Perf defines a function to get durations of callback instances for a given callback objects~\href{https://github.com/azu-lab/ROS2-E2E-Evaluation/blob/main/autoware_perf_galactic/tracetools_analysis-galactic_add_tp/tracetools_analysis/analysis/callback_duration.ipynb}{(Autoware\_Perf/../callback\_duration.ipynb~\faicon{github})}.
    \item \textbf{Latency} is the time a ROS-based system takes to react to a stimulus from the test orchestrating apparatus. Often, field tests include a centralized computer orchestrating the test cases execution and information collection, latency in such cases tends to be significant. Autoware\_Perf illustrates how latency can be computed with an example of a ROS 2 service, where they send a goal to the robot and calculate the time for a response~\href{https://github.com/azu-lab/ROS2-E2E-Evaluation/blob/main/autoware_perf_galactic/tracetools_analysis-galactic_add_tp/tracetools_analysis/analysis/galactic/e2elatency.ipynb}{(Autoware\_Perf/../e2elatency.ipynb~\faicon{github}))}.
    \item \textbf{Synchronization time} is the time taken for a ROS-based system involving more than one robot to share information.
    \item \textbf{Sensor Data Processing time} is the time taken to transform raw sensorial input into information ready to be used by reasoners or planners. Lewis et al. conclude that it is difficult to predict how long robots might have to wait between measurements since quantifying data collection for real-time systems needs to account for all the [metereological] sensors and their respective response times\cite{lewis:2022}
    \item \textbf{Fault Detection and Recovery time} is the time taken to prevent safety hazards. Robots, mainly operating in safety-critical scenarios, often have safety mechanisms to prevent hazards. Testing in the field, in general, asks for safety assessment, thus incurring timing overhead. 
    \item \textbf{Power Management time} is the time taken to prevent stop or graceful degradation due to a power outage. Robots may rely on batteries or other embedded power sources (such as solar panels). Power management may affect the testing conditions and be considered when testing in the field. For example, to start a recharging process in the middle of the mission or to slow the velocity to recharge the batteries using solar energy.
\end{itemize}

\subsubsection{Strengths} Identifying timing constraints is a good practice to avoid neglecting important real-time requirements during development. It also helps isolating the tested behavior without unintended outcomes due to real-time faults. %There is support for formal modeling, including timing variables ready to use.

\subsubsection{Weaknesses} Specifying timing constraints may be complex due to the ROS nature presenting interconnected components and dependencies. There is a lack of standardization or best practices for specifying such properties. This may result in an overhead when the application is not real-time critical. Property specification guidelines (SDB1, SDB2) will further investigate this issue. 

\subsection{CI2. Identify security and privacy constraints}\label{sec:CI2}

\subsubsection{Context (WHEN)} Runtime assessment introduces challenges to security and privacy preservation. Modifying the source code to facilitate testing may, however, open space for security and privacy exploitation\cite{bertolino:2021}. %The developers should specify how ROS-based applications may be secure during testing. 
%A solution to privacy and security is designing testable units with specific features to ease testing and exposing internal information for guaranteeing a given level of security and privacy. 
From the point-of-view of runtime verification, security and privacy preservation revolves around specifying flavors of integrity, confidentiality, and availability\cite{falcone:2021}. For instance, Autonomous Driving Vehicles (ADVs) regulators define policies given the territory they are being used in. However, ADS introduction also requires public trust, w.r.t security and safety~\cite{luckcuck:2019}. In a scenario of runtime assessment, be it field-based testing or runtime verification, security and privacy exploits may be catastrophic. Yet, security is still under-explored when it comes to architectural designs for ROS-based applications~\cite{malavolta2021mining}.
 
\subsubsection{Reason (WHY)} Security and Privacy are often under-explored in the design of ROS-based applications. Threats to privacy and security may be catastrophic and may be an unacceptable side-effect of runtime assessment of such robotic applications. 

\subsubsection{Suggestion (WHAT)}%The development team should identify the security and privacy constraints that may pose a risk to participants' integrity, confidentiality, and availability.
The development team should identify security or privacy vulnerabilities that may pose a risk to participants' integrity, confidentiality, and availability, that may be caused by the testing and runtime verification activities. The ros-security workgroup{\color{red}, in collaboration with Alias Robotics,}\footnote{Deleted after follow-up questionnaire on April 14th.} maintains SROS (git: ros2/sros2) for the analysis of such vulnerabilities and fixes. In addition, Alias Robotics maintains a database of vulnerabilities detected in ROS applications (git: aliasrobotics/RVD) as a means of awareness.

\subsubsection{Process (HOW)} Jeong S. Y. et al.~\cite{jeong2017study} list a set of vulnerabilities typically encountered in ROS applications, including broken authentication, the rosbag replay attack, and service hijacking. Neither preparing the code for runtime assessment nor the runtime assessment procedure itself should enable or facilitate the exploitation of such vulnerabilities. The developers must be aware of such vulnerabilities and specify constraints specific to the domain of the application, enforcing or informing the testing of the danger. From one side, the ros-security working group works on mitigating security vulnerabilities provided by design from ROS~\cite{mayoral2022sros2}. From another stance, other approaches focus on confidentiality, integrity, and availability while providing means to specify control access policies and generate firewall rules based on the fundamental elements of ROS~\cite{hu:2019,huang:2014}.

\subsubsection{Exemplars}~\\ 
FAST-DDS is the current technology used in ROS 2\footnote{Details on FAST-DDS~\href{https://fast-dds.docs.eprosima.com/en/latest/fastdds/security/security.html}{https://fast-dds.docs.eprosima.com/en/latest/fastdds/security/security.html}}. FAST-DDS enables features such as authentication of domain participants using a Certificate Authority (CA), access control to constrain specific operations, authenticated encryption following the Authentication Encryption Standard (AES), logging security events, and data tagging by enabling security labels to data.
In addition, the ros-security working group, in tandem with Alias Robotics, works on SROS, a tool for securing ROS within the DevOps model (\href{https://github.com/ros2/sros2}{ros2/sros~\faicon{github}})~\cite{mayoral2022sros2}.

Hu et al. specify security properties of ROS-based systems~\cite{hu:2019}. The specified security properties follow the definition of a composite of attributes on confidentiality, integrity, and availability, according to Avizienis~\cite{avizienis2004basic}. Hu et al. define the properties following two scenarios: (i) attackers get access to a ROS node and freely allocate memory until reaching an out-of-memory state, (ii) topics or services are hijacked, and the information flowing between ROS nodes is changed to provoke a failure. In such scenarios, the developer's team should specify constraints to the runtime assessment procedure placing a barrier to facilitating the control of ROS nodes in such a way that enables free memory allocation and should specify conditions to allow ROS topics and services remapping without any certification, for instance. The testing team may want to assess whether their runtime assessment will open up exploit opportunities given a set of constraints.

ROSRV, a runtime verification framework for safety and security properties of ROS-based applications, provides a specification language for access control policies and enforces them at runtime~\cite{huang:2014}. Such access control policies may prevent the system from exploiting security breaches, such as enabling the control of safety-critical nodes to the application. More specifically, ROSRV provides access control specifications based on a user-provided specification of access policies using text file inputs. The policies are defined under five categories: groups, nodes, publishers, subscribers, and commands. Nodes represent node names and machine identities, publishers/subscribers define topic names and node identity associated, and commands define the access policy, e.g., full access, localhost (\href{https://github.com/cansuerdogan/ROSRV/blob/master/docs/Usage.md}{ROSRV\faicon{github}}). 

\subsubsection{Strengths} Identifying security and privacy constraints can help protect participants and resources during runtime assessment. This guideline encourages developers to consider security and privacy early on in the design process, rather than as an afterthought. It encourages the development of more secure and trustworthy ROS-based applications and runtime assessment of ROS-based applications, which can improve public trust and acceptance.

\subsubsection{Weaknesses} The guideline, intentionally, does not provide specific details on how to implement security and privacy constraints, leaving it up to the developers to decide which constraints are necessary and how to enforce them, since this is domain-dependent. It may be challenging to understand the various security vulnerabilities associated with ROS-based applications, making it difficult to specify appropriate security and privacy constraints. The guideline may require additional time and resources to implement security and privacy constraints, which may delay the development process. {\color{blue} Systems with lower technology readiness level, such as academic prototypes, may not need a thorough security assessment, making this guideline irrelevant in those cases.}\footnote{Added after follow-up questionnaire on April 14th.}

\subsection{CI3. Identify safety constraints} \label{sec:CI3}

\subsubsection{Context (WHEN)} The assessment of safety constraints is essential for both runtime verification and field-based testing. When stimulating robotic systems with extreme scenarios, for instance in robustness testing~\cite{afzal:2020}, it's crucial to consider potential threats to personnel and the properties being tested. These threats limit the ability to conduct online assessments for safety-critical applications, particularly in robotics. To ensure the benefits of field-based testing~\cite{bertolino:2021}, it's important to carefully address and compensate for the introduced safety risks. Non-negotiable safety constraints should be maintained throughout the confidence-gathering process, as they determine the readiness and release of technology, both in industry and everyday use~\cite{bozhinoski2019safety}.

\subsubsection{Reason (WHY)} Safety hazards may unable runtime verification or field-based testing since corner cases may pose threats to testing personnel or damage property during runtime assessment.

\subsubsection{Suggestion (WHAT)} %The developers should identify safety constraints to prevent personnel or proprietary damage during runtime assessment.
The developers should identify the boundaries of a safe behavior (i.e., safety constraints) to enable the use of mechanisms for preventing the robot from hurting operators or property during testing and verification activities. For example, the developers can identify constraints like speed limit, distance to obstacle, or conditions for emergency stop, which can be used by monitoring tools like ROSMonitoring (git: autonomy-and-verification-uol/ROSMonitoring), or used by an independent safety controller in a separate ROS node to prevent the robot from falling from a cliff, e.g., the Kobuki robot (git: yujinrobot/kobuki).    

\subsubsection{Process (HOW)} Safety constraints may be specified in using many specification languages. The known toy example in mobile robotics, Kobuki, specifies safety properties in a separate ROS node using the switch-case in Python; Adam et al.\cite{adam2014towards} proposes rule-based specifications in the format of boolean equations that predicate over messages over topics; Stadler et al.~\cite{stadler2023romosu}, uses an event processing language offering query-based operations; Finally, Huang et. al~\cite{huang:2014} enables the specification of temporal properties leveraging monitoring-oriented programming (MOP).

\subsubsection{Exemplars}~\\ 
\textbf{Typical safety constraints:}
\begin{itemize}
    \item emergency stop \cite{adam2014towards}
    \item speed monitoring (e.g., $v < 0.2m/s$)~\cite{adam2014towards}, and \\movement speed limit (e.g., speed limit $0.35 m/s$)~\cite{stadler2023romosu}
    \item timing monitoring (e.g., $t > 10$)~\cite{adam2014towards}
    \item obstacle avoidance (e.g., maintain at least $35cm$ distance from object)~\cite{stadler2023romosu}
    \item joint effort (e.g., \href{https://github.com/MStadler-Organization/ROMoSu/blob/main/services/constraint_engines/src/main/resources/constraints/c1_mx_joint_effort.cst}{max\_joint\_effort\faicon{github}})~\cite{stadler2023romosu}
\end{itemize}
\textbf{Technologies:} 

The Kobuki robot implements a safety controller (\href{https://github.com/yujinrobot/kobuki/blob/23748ed3dfb082831ca8eaaef1a0b08588dbcb65/kobuki_safety_controller/include/kobuki_safety_controller/safety_controller.hpp}{\faicon{github}}). The kobuki's safety controller specifies, using Python at code-level, a state machine ensuring that the robot stops whenever it is close to a cliff, the bumper sensor was pressed, or at least one of the wheels dropped (or was raised in the air). The Kobuki's safety controller is a separate ROS node collecting bumper, cliff and wheel events. A sequence of events may trigger an alert or issues velocity commands to deviate Kobuki from the threat.

Adam S. et al.~\cite{adam2014towards} defines a rule-based language for enforcing safety constraints on existing ROS-based software. Their approaches uses a simplified metamodel to describe the ROS software enabling static analysis as well as invariant monitoring. The authors explain that separating the specification of safety issues from functionality facilitates attesting that the robotic behavior conforms to safety requirements. Their rule-based approach enables the specification of actions that preclude rules encoded in boolean equations (e.g. cmd\_vel\_left $>$ 0.02m/s) over messages in topics.

Stadler et al.,~\cite{stadler2023romosu} uses the Esper Constraint Engine to check for violations of the safety constraints. Such constraints are specified using the EPL notation. Event Processing Language (EPL) is a SQL-standard language with extensions, offering SELECT, FROM, WHERE, GROUP BY, HAVING and ORDER BY clauses. For instance, they specify that an event such as JointEffortEvent (AEvent) will not exceed a maximum of 5.0 in an ESL constraint specification (i.e., \href{https://github.com/MStadler-Organization/ROMoSu/blob/main/services/constraint_engines/src/main/resources/constraints/c1_mx_joint_effort.cst}{max\_joint\_effort\faicon{github}}).

\begin{lstlisting}[language=SQL, caption={Safety constraint in EPL notation.\vspace{.35cm}}]
select * from AEvent(MaxValue > 5.0)
\end{lstlisting}

Huang et al.'s~\cite{huang:2014} monitoring infrastructure enables the use of any logic plugins of Monitoring-Oriented Programming, thus enabling specification of temporal properties over events, such as regular expressions, linear temporal logics, and context-free grammars. For instance, one of their monitors predicates on the position of the turret installed in the autonomous vehicle, i.e., ``the gun should not exceed a maximum joint angular position otherwise the turret targets itself.''.

\subsubsection{Strengths} By identifying safety constraints, developers can demonstrate compliance with these requirements, providing assurance to stakeholders that appropriate safety measures are in place. Early detection and response to safety violations, such as exceeding speed limits or approaching obstacles too closely. This early detection and response can help prevent accidents and minimize potential damage.

\subsubsection{Weaknesses} Identification of safety hazards involves understanding the system's behavior, identifying potential risks, and formulating appropriate constraints. This process can be time-consuming and complex, especially for large and intricate systems, potentially increasing development costs. 

\subsection{CD1. Developers should strive for ROS nodes with single responsibility}\label{sec:CD1}

\subsubsection{Context (WHEN)}
ROS fosters a rich toolkit for designing modular robotics software~\cite{limsoonthrakul2009modular}.  Developers face design decisions of how to implement a given set of requirements using ROS fundamental concepts, i.e., nodes, topics, services, packages~\cite{malavolta2021mining}. In order to facilitate runtime assessment, the system's computational units should be designed such that they can be safely exposed to trials with warrantied no side effects on the running system~\cite{bertolino:2021}. In addition, it should reduce the cost of observing and controlling modules, or, in robotics, atomic actions (or skills)~\cite{efatmaneshnik2017study}.

\subsubsection{Reason (WHY)} Mapping functional units to ROS nodes enables fine-grained observation and control of the robotic behavior.

\subsubsection{{Suggestion} (WHAT)} %To facilitate runtime assessment and enable fine-grained observation and control, the developers should implement ROS nodes following the single responsibility principle.
To facilitate assessment during the robot operation and enable fine-grained observation and control, the developers should implement ROS nodes following the single responsibility principle (i.e., each node should implement a single feature and different nodes can be combined to perform a complex task). For example, developers should implement independent nodes for path planning and reactive manoeuvring, or independent nodes for defining primitive skills like grasping an object or simultaneous localization and mapping (SLAM).

\subsubsection{Process (HOW)} We divide the means to designing ROS nodes with single responsibility in two: hierarchical design, and skill-based design. In hierarchical design, ROS nodes are organized based on the goals they achieve, with each node responsible for a specific task or functionality\cite{hartsell:2019,Gil2021}. This approach allows for clear separation of responsibilities and easier maintenance. In skill-based design, ROS nodes are organized based on the skills they possess, with each node responsible for a specific capability or behavior\cite{rovida2017skiros,rodrigues2022architecture,albore2023skill}. This approach enables more flexibility and reusability of nodes, as they can be combined to perform various tasks.

\subsubsection{Exemplars}~\\ 
\textbf{Hierarchical design.} Hartswell et al. define components as building blocks that may be hierarchically composed to fulfill the system's functional requirements~\cite{hartsell:2019}. Their running example implements ROS nodes with complementary but distinct, and independent, functionalities. One node resolves path planning in a deliberative control setting, and the other is responsible for the low-level PID controller reactively manoeuvring the robot. 
In the healthcare domain, the Body Sensor Network (\href{https://github.com/lesunb/bsn}{lesunb/bsn\faicon{github}}) defines ROS nodes after concrete tasks that, composed, should fulfil the system's goal. Tasks such as collecting SPO2 data, collecting heartbeat data, fuse data, or identifying emergency~\cite{Gil2021}. For instance, the collect SPO2 data task implements an independent node for collecting, filtering, and transferring data~\href{https://github.com/lesunb/bsn/blob/master/src/sa-bsn/target_system/components/component/src/g3t1_1/G3T1_1.cpp}{\faicon{github}}. Given that each sub-task (i.e., collecting, filtering, and transferring) is strictly dependent on each other, yet, should not depend in the environment and together form an atomic behavior. Separating the sub-tasks in different nodes may render incomplete test cases that are hard to read and often meaningless.\\  
\textbf{Skill-based design} typically defines skills as fundamental software building blocks operating a modification on the world stage. In such approaches, skills should be modular and reusable. Although ROS nodes provide a natural means for modular design, it is not common to map skills to nodes in current skill-based designs. For instance, SkiROS~\cite{rovida2017skiros} implements 3 nodes: World Model Manager, Task Manager, Skill Manager (\href{https://github.com/RVMI/skiros2/blob/de00abafffe78c8da6ba35e8259d6ad075ec72b6/skiros2_skill/src/skiros2_skill/core/skill.py#L622}{skiros2\_skill\faicon{github}}). In addition, HRMS~\cite{rodrigues2022architecture} does not map skills to nodes. It builds skills that under the Behavior Trees notation may reuse existing nodes (\href{https://github.com/Gastd/py_trees_ros_behaviors/tree/devel/py_trees_ros_behaviors}{hmrs/skills\faicon{github}}). Lack of standard mapping from skills to actual computation impairs the verification of skill-based approaches at skill level.
Towards verifiable ROS-based applications, a promising architecture, namely RobMoSys\footnote{\href{https://robmosys.eu/wiki/general_principles:separation_of_levels_and_separation_of_concerns}{https://robmosys.eu/wiki}}, suggests separation of concerns between different levels such as Mission, Task Plot, Skill, Service, Function, whereas Skill concerns to configuration, e.g., grasp object with constraint, and functions concern to computation, e.g. inverse kinematics solver. In this direction, Albore A. et al.~\cite{albore2023skill} promote ROS2 code generation whilst mapping skillsets to ROS nodes with a single responsibility.

\subsubsection{Strengths} Modularity enables fine-grained observation of system requirements. In addition, it caters to clear interfaces for runtime inspection and allows for mocking and substituting behavior for assurance scenarios.

\subsubsection{Weaknesses} Feedback loops, however, may impair testing, i.e., modularity turns out to be costly for systems with feedback loops, whereas the system's behavior is context-dependent~\cite{hutchison2018}.

\subsection{CD2. Ensure global time monotonicity of events and states}\label{sec:CD2}

\subsubsection{Context (WHEN)} 
As distributed systems, such as ROS-based applications, rely on time scheduling for their operation, ensuring time monotonicity is crucial to guarantee the replicability and reproducibility of test cases. Non-determinism in the scheduling of events can lead to unexpected behavior, compromising the reliability of tests and hindering their reproduction. To address this issue, developers must ensure that the testing team is aware of the expected behavior given the occurrence of events, which requires establishing a clear execution order and priority. For instance, by synchronizing different types of data at package or subscription-level~\cite{malavolta2021mining}.

\subsubsection{Reason (WHY)} Ensuring global time monotonicity of events and states permits to address the potential non-determinism in the scheduling of events in ROS-based applications. %, which can compromise the reliability of tests and hinder their reproduction. By ensuring time monotonicity, developers can promote the reliability of tests and facilitate the reproducibility of results in such systems. 

\subsubsection{Suggestion (WHAT)} %The development team should ensure global time monotonicity of events and states to avoid potential scheduling non-determinism.
The development team should ensure global time monotonicity of events and states to avoid potential non-determinism in scheduling. Such non-determinism is a threat to getting confidence in the system since repeated tests under the same conditions may turn into different results. A technique that can be used to ensure determinism is annotating messages and requests with timestamps and implementing a logical time synchronizer, similar to what is done by MAVROS (git: mavlink/mavros). Also, the Time Synchronizer message filter (wiki: message\_filters) may be used for this purpose.
    
\subsubsection{Process (HOW)}  Events are said to be monotonic in time whenever for a set of events scheduled over a global clock, two consecutive events are successive. First the developers should understand how events are scheduled and the limitations of the application towards predictable ordering of events~\cite{chaaban2023new,choi2021picas}. Then, the developers should analyze and guarantee that all processes are executed in the expected order and will lead to predictable behavior. Developers may accomplish such analysis and guarantee provision with external tools, for instance, formal methods~\cite{blass2021ros,halder2017formal} or by embedding timestamps (e.g., SteadyTime) and filtering messages to guarantee ordered events (e.g., MAVROS).

\subsubsection{Exemplars} ~\\
\textbf{Understand the scheduling of ROS events and states.} 
Chaaban K.~\cite{chaaban2023new} explains that ROS 2 schedules callbacks using a non-preemptive algorithm that consumes messages depending on their type. Unlike typical real-time priority-based scheduling algorithms, ROS 2 does not execute callbacks in their activation instances. Thus non-time-based messages are scheduled in a round-robin fashion. To this extent, ROS 2 (which claims to address real-time) presents limitations when asked for well-defined execution orders and priority inversion. Choi et al. ~\cite{choi2021picas} promotes \href{https://github.com/rtenlab/ros2-picas}{rtenlab/ros2-picas~\faicon{github}}, a new scheduling algorithm that adds priority awareness for scheduling in ROS2.\\
\textbf{Analyse starvation-freedom to support monotonicity.}
%\ric{i am concerned about the strength of this argument. does starvation-freedom correlates to monotonicity? in what way?}
Bla{\ss} T. et al.~\cite{blass2021ros} proposes a response-time analysis exploiting the round-robin properties. The authors present an analysis of starvation-freedom using three techniques: modeling processor demand as execution-time curves instead of scalar worst-case execution times (WCETs), accounting for the effects of quiet times and busy windows in the activation curve derivation, and exploiting the round-robin behavior of the ROS callback scheduler. Starvation freedom indicates monotonicity and ordering of events, it helps the developers to understand real-time behavior and set expectations.
Halder R. et. al~\cite{halder2017formal} use model checking (e.g., UPPAAL~\cite{uppaal1996}) to analyze real-time behavior in ROS-based applications. Under the claim that ROS non-deterministically empties the communication queues, the authors focus on modeling the message-passing behavior of ROS and verifying whether the queue overflows. Since overflow here means that some process is starving, thus the application is not monotonic in time. The authors offer the models in timed automata and TCTL (Temporal Computational Tree Logic) properties designed to ensure real-time for the safety controller of the Kobuki\footnote{\url{http://wiki.ros.org/kobuki}} exemplar.\\ 
%Aware of the issue of checking real-time properties using traditional model checkers (i.e., scalability), Hu et al.~\cite{hu:2019}, use the clock ticks to discretize time and check properties at runtime. %%It happens that hu et al, doesnt really solve the real-time problem. they point ouut that it is an issue and discretize the time using clock ticks.
\textbf{Annotating messages with timestamps and synchronization to guarantee ordering.}
The SteadyTime\footnote{\href{https://design.ros2.org/articles/clock_and_time.html}{https://design.ros2.org/articles/clock\_and\_time.html}} class in ROS represents a monotonic clock, functioning independently of physical time and with steady tick times. MAVROS~(\href{https://github.com/mavlink/mavros}{mavlink/mavros~\faicon{github}}), a library broadly used in ArduPilot %~\cite{ArduPilot} 
for flight control, approaches time monotonicity guarantees by implementing a logical time synchronizer. The synchronizer ensures that the time passing in MAVROS is aligned with the time on ArduPilot's side, avoiding drifts that could lead the application to fail. More importantly, the time synchronizer uses a particular type of message that embeds timestamps for clock synchronization for updating ArduPilot about its time status~\href{https://github.com/mavlink/mavros/blob/ros2/mavros_msgs/msg/TimesyncStatus.msg}{(TimesyncStatus.msg~\faicon{github})}. Messages such as this can be used for synchronizing the occurrence of events in the system. 
The Time Synchronizer message filter\footnote{\href{http://wiki.ros.org/message_filters}{https://wiki.ros.org/message\_filters}}, for example, reads timestamps from the header of messages and synchronize message by outputting channels to a single callback.\\ 
\subsubsection{Strengths} Tests reliability increases by enabling the prediction of the expected behavior of a system under scrutiny. In addition, time monotonicity guarantees can facilitate reproducing test results by establishing a clear execution order and priority. Finally, developers can reduce the time taken and resources used to verify the system behavior by implementing time synchronization and annotation messages with timestamps.\\ 
\subsubsection{Weaknesses} Implementing time synchronization to ensure time monotonicity may require additional development effort, adding complexity to the system. Also, time synchronization may add performance overhead due to additional operations execution. Achieving real-time behavior depends on the (interaction with the) operating system. %\gena{Is this feature also dependent on the (interaction with the) operating system?}

\subsection{I1. Provide an API for querying and updating internal lifecycle} \label{sec:I1}

\subsubsection{Context (WHEN)} Autonomous systems, such as robotic applications, often require stateful compute nodes~\cite{hutchison2018}. However, the internal states within ROS nodes are typically hidden and not easily accessible, limiting the ability to diagnose and understand unexpected behavior. Exposing these hidden states is crucial for providing granular information on the system's behavior, rendering increased observability. Furthermore, managing these hidden states allows for actions such as starting, stopping, and rolling back to a specific state, in other words, increased controllability. The running system should be both observable and controllable~\cite{falcone:2021, bertolino:2021}, as these states can be application-specific and not standard~\cite{malavolta2021mining}.

\subsubsection{Reason (WHY)}  The use of ROS nodes with lifecycle management can facilitate testing by providing a structured way to manage the state of the nodes and the interactions between them. This structure helps to ensure that nodes are in the right state for testing and that the interactions between nodes are predictable. Furthermore, it helps mitigate dangling references to nodes that are no longer in use.% \gena{there might be another issue: concurrency and dangling references to nodes no longer 'alive'. the latter is especially critical in embedded systems, I believe.}

\subsubsection{Suggestion (WHAT)} %To facilitate field-based testing, the development team should adopt custom lifecycle conventions and prepare an API for querying and updating the internal nodes' life-cycle.
 To facilitate field-based testing, the development team should properly manage the ROS nodes' lifecycle and prepare APIs for querying and updating the internal nodes' life-cycle, e.g., to ensure that nodes are in the right state for testing. For example, developers can use modes (git: ros2/demos) for lifecycle management. In the context of Micro-ROS (git: micro-ROS), developers can define custom lifecycle modes (git: micro-ROS/system\_modes)  like sleep, power saving, starting, processing, and ending modes, and use separate extra nodes for mode monitoring and mode update.
    
\subsubsection{Process (HOW)}  The team should define a custom life-cycle for the ROS-based application, for instance, the life-cycle phases could be: starting, processing, and ending~\cite{conte:2018}, using system\_modes from Micro-ROS\cite{belsare2023micro}. Moreover, the processing phase can further be divided into waiting and executing steps and application-specific states, and the transitions between phases should be well-defined by events. The development team should then prepare an API for managing the life-cycle of nodes~\cite{nordmann2021system}, which can be queried or updated through ROS interfaces, such as the client-server interface. The API should allow for the representation of all nodes in the application, which can be queried or updated using the interface.

\subsubsection{Exemplars}~\\ 
\textbf{Customized life-cycle}
Conte G. et al.~\cite{conte:2018} define a custom life-cycle in ROS for their autonomous surface vehicle. The life cycle has three phases: starting, processing, and ending. The processing phase can be subdivided into two other: waiting and executing. Events define the transition between phases. The authors claim that such organization helped in the field testing when they had to explicitly shut down a (ROS) agent, shut down the agency infrastructure, or detect a failure in the ROS infrastructure. ROS2 provides the concept of life-cycle by design. Developers may inherit from the LifecycleNode from rclcpp to enable the standardized life-cycle management from ROS2. Belsare K. et al.~\cite{belsare2023micro}, namely \href{https://github.com/micro-ROS}{Micro-ROS~\faicon{github}}, extends the ROS2 life-cycle to the domain of embedded systems. Their extension enables the specification of (sub-)systems or systems-of-systems in a hierarchical finite-state machine style. It creates the concept of modes within the active state. System modes (\href{https://github.com/micro-ROS/system_modes}{micro-ROS/system$\_$modes~\faicon{github}}) are customizable and can be used to track sleep modes and power saving~\cite{nordmann2021system}. The authors present an example (\href{https://github.com/micro-ROS/system_modes/blob/master/system_modes_examples/src/manipulator.cpp}{micro-ROS/system$\_$modes/system$\_$modes$\_$examples~\faicon{github}}) of how can add {\em weak} and {\em strong} as customized modes for an active manipulator.\\ 

\begin{lstlisting}[language=SQL, caption={YAML definition of custom system modes weak and strong for torque control.\vspace{.35cm}}]
    manipulator:
      ros__parameters:
        type: node
        modes:
          __DEFAULT__:
            ros__parameters:
              max_torque: 0.1
          WEAK:
            ros__parameters:
              max_torque: 0.1
          STRONG:
            ros__parameters:
              max_torque: 0.2
\end{lstlisting}
    
\textbf{Life-cycle management} is the ability to query and update the nodes' life-cycle. \href{https://github.com/ros2/rclc/tree/master/rclc_lifecycle}{rclc/rclc$\_$lifecycle~\faicon{github}} the library used by ROS2 provides the functionalities to managing nodes using the ROS2 stack~\cite{staschulat2020rclc}. rclc$\_$lifecycle implements a ROS node that represents all other ROS nodes within the application. The nodes encode finite state machines that can be queried or updated using the ROS service interface. The lifecycle$\_$talker example (\href{https://github.com/ros2/demos/blob/foxy/lifecycle/src/lifecycle_service_client.cpp}{ros2/demos/lifecycle~\faicon{github}}) illustrates how the get$\_$state and change$\_$state services query or update the life-cycle. The ROS2 implementation, however, does not support hierarchical states. To mitigate the problem,  \href{https://github.com/micro-ROS}{Micro-ROS~\faicon{github}} defines two extra nodes, the mode monitor node and the mode manager node~\cite{nordmann2021system}. The mode monitor infers the state (i.e., mode) of underlying nodes; The mode manager may use the (inferred) state to update modes of sub-systems, modes of nodes, and node parameters.

\subsubsection{Strengths} Following this guideline results in reliable and repeatable runtime assessment since the life-cycle manager can ensure that the application is in the desired state. Moreover, it is easier to setup and teardown testing harnesses since it would be possible to understand the current state of the application, avoiding interruptions in critical phases, and planning for start and stop in the appropriate time.

\subsubsection{Weaknesses} As a drawback, there will be overhead associated with meta-data for life-cycle management, and increasing the number of lines of code may impact the system's latency. Also, custom states may ask for larger models representing the possible life-cycle and management, incurring in cost of modeling and maintenance. 

\subsection{I2. Provide an API for logging and filtering}\label{sec:I2}

\subsubsection{Context (WHEN)} Dynamically gathering information is a fundamental step for gaining confidence in ROS-based systems. Logging (and playback) is, in fact, one of the most used techniques for testing ROS-based systems~\cite{afzal:2020}. Often named \textit{monitoring}~\cite{falcone:2021}, or \textit{logging}~\cite{bertolino:2021}, the process of recording textual or numerical information about events of interest may be a valuable input to the testing team. With such data in hand, the testing team will process the data and transform it into useful information to challenge their hypotheses about how the system should work.
%\gena{I have the impression this guideline has a bit of overlap with D2. I may be wrong though....}

\subsubsection{Reason (WHY)} Logging important events depends on instrumenting the code (with `hooks') that enables the information retrieval activity. It is unrealistic to assume that the testing team will have access to the source code or that the testing team knows what events to log or how to do so.

\subsubsection{Suggestion (WHAT)} %The development team should provide an API for logging and filtering data to facilitate access to valuable runtime data.
The development team should provide an API for logging and filtering data to enable access to valuable runtime data which should be used for both runtime verification and field-based testing. The standard approach to logging and filtering is rosbag (wiki: rosbag). Though, in addition, AWS CloudWatch (git: aws-robotics/cloudwatchlogs-ros2) collects data from the rosout topic and provides a filter for eliminating noise from the logged events. Another example is the Robotic Black Box (git: ropod-project/black-box) which allows for listening to data traffic from distinct sources and logging the messages using MongoDB.

\subsubsection{Process (HOW)} We divide, according to Falcone et al.~\cite{falcone:2021}, techniques for gathering information in two: inline, and outline. Inline logging and filtering stand for techniques that ask for actually inserting snippets of code in the system under scrutiny as a means to provide an API for logging, e.g.,~\cite{kaveti2021ros}. Outline logging and filtering stands for techniques that enable an external means to gather and filter information that does not require changing the source code, e.g.,~\cite{ferrando:2020,elbaum2000software,mitrevski2022deploying}. Developers may choose one or another given their domain of application.

\subsubsection{Exemplars}~\\ 
\textbf{Inline logging and filtering.} ROS, by standard, contains a system-wide string logging mechanism, namely ROS logging (\href{http://wiki.ros.org/roscpp/Overview/Logging}{http://wiki.ros/logging}). ROS logging works with a set of macros defined for instrumenting the nodes with information hooks. In the background, the macros send messages with the information to be logged through a standard topic called rosout. On the other side of the topic, an extra node, within the roscore package, persists the data in a textual format (\href{https://github.com/ros/ros_comm/blob/noetic-devel/clients/rospy/src/rospy/impl/rosout.py}{ros/../rosout~\faicon{github}}). Developers can use the macros to log information that might be used for testing in a later stage, given the application-specific requirements. For instance, the Amazon AWS service for robotics provides AWS CloudWatch Logs (\href{https://github.com/aws-robotics/cloudwatchlogs-ros2}{aws-robotics/cloudwatchlogs-ros2~\faicon{github}}) interfaces directly with rosout to monitor applications using the standard ROS logging interface. In addition, the standard library provides logging macros with embedded filtering capabilities, which enables eliminating noise from the logged events and can render a useful tool for testers.
ROS Rescue~\cite{kaveti2021ros} is another example of inline logging. The tool aims at solving the problem of ROSMaster as a single point of failure. The authors approach check-pointing and restoring state by logging changes in the metadata stored in the master node. Such metadata contains URIs from various nodes, port numbers, published or subscribed topics, services, and parameters from the parameter server. Kaveti P. et al. create an API for the ROS master node (\href{https://github.com/PushyamiKaveti/fault-tolerant-ros-master/blob/master/src/ros_comm/rosmaster/src/rosmaster/master_api.py}{master\_api.py~\faicon{github}}) using the official logging library from Python\footnote{\href{https://docs.python.org/3/howto/logging.html}{https://docs.python.org/3/howto/logging.html}}~to persist metadata in YAML format. Their technique opens space for further inspection of ROS applications without access to the source code.\\ 
\textbf{Outline logging and filtering.} ROSMonitoring~\cite{ferrando:2020} employs monitors to persist events in textual format. The monitors contain filtering capabilities to eliminate entries that are inconsistent with the specification (requires an oracle). In this context, the launch files to configure ROSMonitoring can be seen as an API for logging and filtering (\href{https://github.com/autonomy-and-verification-uol/ROSMonitoring/blob/master/generator/online_config.yaml}{ROSMonitoring/../online\_config.yaml~\faicon{github}}). Monitors in ROSMonitoring are nodes, thus, the API is a set of known topics and message formats. The tester, in that case, only needs to specify what topics ROSMonitoring will listen to and the type of message to be recorded. The logging and filtering happen within a separate service. On a similar stance, and inspired by aircraft black box (and software black box~\cite{elbaum2000software}), Mitrevski, et al.~\cite{mitrevski2022deploying} proposes the concept of Robotic Black Box (\href{https://github.com/ropod-project/black-box}{ropod-project/black-box~\faicon{github}}). The black box operates as an isolated component responsible for listening to data traffic from distinct sources and logging in an easily retrievable medium. Similarly to ROSMonitoring, Mitrevski's black box approach to logging (\href{https://github.com/ropod-project/black-box/blob/master/pybb/logger_main.py}{ropod-project/black-box/../logger\_main.*~\faicon{github}}) inspects topics and message types that are configured in advance. Different from ROSMonitoring, Robotic Black Box offers logging not only in textual format but also in a MongoDB database, which is essentially useful for data processing, filtering, and retrieval. Robotic Black Box stands out when it comes to its filtering and retrieval capabilities. The approach builds a customized query interface over the MongoDB database using names of collections, timestamps and metadata to filter the results (\href{https://github.com/ropod-project/black-box-tools/blob/master/black_box_tools/db_utils.py}{black\_box\_tools/db\_utils.py~\faicon{github}}).
%Black box paper: \href{https://arxiv.org/pdf/2206.12719.pdf}{arxiv}.  \href{https://github.com/ropod-project/black-box}{ropod-project/black-box~\faicon{github}} \ric{maybe talk to argentina to get som insight} \ric{also, look at \href{https://www.fabiodisconzi.com/open-h2020/projects/206247/deliverables.html}{deliverables robustness and dependability}}

\subsubsection{Strengths} An API for retrieval and filtering facilitates access to valuable information resulting in effortless observability of inner states and events. %It also supports the testing team in not having to modify the source code to test maintaining encapsulation. \gena{Not sure I understand the last strength. No logging no runtime verification, as I see it. This might be one of the most important for verification purposes.}

\subsubsection{Weaknesses} Overuse of logging may result in performance issues. Incorrectly implemented logging and filtering capabilities may lead to noise in the data, impacting the reliability of the tests. Finally, insufficient logging may result in an incomplete assessment of the system behavior and might generate false positives.

% 23-04-24 11:18
\subsection{I3. Provide an API for injecting faults in execution scenarios}\label{sec:I3} 

\subsubsection{Context (WHEN)} Stimulating ROS-based systems with unexpected scenarios is a cornerstone of gathering confidence in the system's robustness~\cite{afzal:2020,hutchison2018}. Such unexpected scenarios either emerge from faults in the robot's control logic or unforeseen inputs unfolding from complex interactions with the environment. Therefore, preparing the ROS-based systems to systematically explore unintended behavior and complex environmental interactions becomes important in runtime verification~\cite{falcone:2021} and field-based testing~\cite{bertolino:2021} for robust ROS-based applications. Fault injection and error emulation are the two fundamental approaches to systematically stimulating a computing system with unexpected scenarios for confidence-gathering purposes~\cite{duraes2006emulation}.

\subsubsection{Reason (WHY)} Providing an API for stimulating unexpected scenarios for testing the robustness of the target system can help address challenges in finding both fault and error sets representative of real software faults. 

\subsubsection{Suggestion (WHAT)} 
To enable runtime verification and field-based testing, developers should provide an API for injecting faults or emulating runtime errors. For instance, to emulate the consequences of software faults, ros1-fuzzer (git: aliasrobotics/ros1\_fuzzer) provides an API for ROS messages fuzzing. As another example, to imitate the mistakes of programmers, IM-FIT (git: cembglm/imfit) is a tool for injecting faults in ROS applications.

%The developers should provide an API for injecting faults at source code or emulating runtime errors to facilitate the verification of robustness of ROS-based systems.

\subsubsection{Process (HOW)} There are two identified means to enabling unexpected scenarios injection in ROS: providing an API fault injection and or an API for error emulation. The two methods differ concerning their assumptions. Fault injection is about changing the source code and requires knowledge about the system's internal structure (e.g., imfit~\cite{yayan2023}). Error emulation is about changing the system during execution and should not require knowledge about the system itself (e.g., ros1\_fuzzer, and ros2\_fuzzer). Thus, from the developer's point of view, enabling faulty scenarios through an API requires deciding whether fault injection or error emulation is the most suitable based on the system's requirements. 

\subsubsection{Exemplars}~\\ 
\textbf{Fault injection.} Fault injection imitates the mistakes of programmers by changing the system under scrutiny's source code~\cite{barbosa2012fault}. Developers can embed an interface for enabling source code modifications to inject faults in the ROS-based system. %This approach asks for an understanding of the system and its objectives.
For instance, IM-FIT(\href{https://github.com/cembglm/imfit}{cembglm/imfit~\faicon{github}}) is a tool tailored to mutation-based software fault injection for ROS applications~\cite{yayan2023}. Listing \ref{lst:mut} describes a subset of the IM-FIT ROS mutations library which offering three operations (delete, change, and external) on defined ROS primitives, such as publishers, subscribers, timers, global variables, namespaces, service clients. Moreover, IM-FIT offers an interface to decide when, where and how the mutators will inflict faults in the source code. Embedding IM-FIT in the project as an API to fault injection facilitates robustness testing for the QA team. %Within the IM-FIT testing pipeline, the testing team should choose when, where, and how the mutators shall inflict faults in the source code. The tool parses the source code of the target system, mutates the source code, deploys it in a docker container and runs tests with the mutations, further dividing them into survived mutators or killed mutators.\\  
%\ric{\cite{hsiao2021mavfi} uses the technique of bitflip to corrupt states at architectural-level \href{https://github.com/harvard-edge/MAVBench/tree/mavfi}{mavfi\faicon{github}}}

\begin{lstlisting}[language=XML, label={lst:mut}, caption={Snippet of the IM-FIT's JSON library containing mutations for fault injection in ROS-based systems.\vspace{.35cm}}]
{"all_faults": [
    {"fault": {
        "Fault_Name": "Subscriber Delete",
        "Target_to_Change": "rospy.Subscriber",
        "Changed": " ",
        "Explanation": "Subscriber deletes"
    }},
    ...
    {"fault": {
        "Fault_Name": "Periodic Timer Change",
        "Target_to_Change": "rospy.Timer",
        "Changed": "rospy.Time",
        "Explanation": "Periodic timer is wrong"
    }},
    ...
    {"fault": {
            "Fault_Name": "External ROS Message",
            "Target_to_Change": "[rospy.Message]{13}",
            "Changed": "rospy.Message rospy.Message",
            "Explanation": "External ROS Message""
    }}
]}
\end{lstlisting}
\textbf{API for error emulation}. Error injection attempts to emulate the consequences of software faults by manipulating the runtime states/events of the system under scrutiny~\cite{lenka2018fault}. Developers can embed an interface within the ROS-based system enabling a set of operations to disturb it during runtime. 
%For instance, PostMonkey~\cite{alnawasreh2017online} modifies the source code by introducing a wrapper over the IPC communication channel which can be set up prepares a shell script to alter the testing environment with two operations: send random messages to nodes or delay messages. \ric{Unfortuantely PostMonkey was not developed for ROS neither operates on ROS applications.}
For instance, ros1-fuzzer~\href{https://github.com/aliasrobotics/ros1_fuzzer}{(aliasrobotics/ros1\_fuzzer~\faicon{github})} provides an API for ROS messages fuzzing. The API requests the topic's name, the message type and datatype strategies to fuzzing the message's content. Although the datatype and constraints are hard coded in the API, defining the topic name and message type are done in the command line. For example,  {{\footnotesize \texttt{\$}}| ros_fuzzer -t /rosout -m rosgraph_msgs/Log|}, in which the user is fuzzing a |Log| message sent to the |/rosout| topic. 
The authors evolved ros1-fuzzer to suit ROS 2 applications, resulting in ros2-fuzzer (\href{https://github.com/aliasrobotics/ros2_fuzzer}{aliasrobotics/ros2\_fuzzer~\faicon{github}}). ros2-fuzzer extends the interface enabling service-level fuzzing, not only message fuzzing as was ros1-fuzzer. The addition affected the API asking for an extra argument (|service| or |message|) in the command, e.g., {{\footnotesize \texttt{\$}}| ros2_fuzzer.py service example_interfaces/AddTwoInts add_two_ints|}.
% RosPenTois a penetration testing tool for ROS-based applications. The tool uses XML remote procedure calls (XMLRPC) to emulate errors due to security breaches in running ROS-based applications. 

\subsubsection{Strengths} Providing an API for fault injection and error emulation with a representative set of possible operations enables balck-box robustness testing. It also may save time for the testing team, which can build scenarios on top of the provided interface.

\subsubsection{Weaknesses} Embedding an interface for enabling source code modifications or runtime disturbances can be time-consuming for developers whenever there are no third-party tools that provide the required operations. This guideline should be avoided when verifying or testing safety-critical systems.

\subsection{I4. Isolate components for testing}\label{sec:I4} 

    \subsubsection{Context (WHEN)} Robotics applications require to be safely field tested with warrantied no side effects on the running system or the environment, including personnel. To this end, it is fundamental to pursue isolation of the components being tested.
    
    %Embedding intermediary nodes to intercept data flowing between nodes is a strategy commonly referred to as Man-in-the-Middle (MITM) and it has proven useful in the robotics domain. 
    Man-in-the-Middle (MITM) can provide isolation of computing nodes for testing, which, as stated by Bertolino et al \cite{bertolino:2021}, can guarantee that the execution of the field tests does not interfere with the operation of the tested system.
    In addition, MITM nodes promotes the ability to drop or modifying internal signals improving the controllability of events and states, which as described by \cite{falcone:2021}, refers to the degree to which a certain specification can be enforced on the system.

    \subsubsection{Reason (WHY)}
    The ROS ecosystem does not provide a native mechanism for node isolation. The MITM node strategy can be a powerful and flexible design pattern to isolate computing nodes in ROS-based systems. It allows for increased visibility into the system's operation, more flexible communication between nodes, and improved reliability and security.
    
    \subsubsection{Suggestion (WHAT)}
    Isolation of components is an important feature to enable field-based testing (by following the ``let it crash" philosophy introduced by Netflix (web:chaos-monkey) while avoiding the crash of the system. Isolation permits catching immediately the component that is crashing and executing countermeasures to keep the system up. Examples of solutions for isolation are: (i) the use of proxy nodes of ROSRV (git: cansuerdogan/ROSRV), or (ii) introducing intermediary nodes between original nodes by exploiting the topic remapping functionality (wiki: remap) of ROSMonitoring (git: autonomy-and-verification-uol/ROSMonitoring), which enables swapping topic names just before running the application.

   %  The QA team should introduce intermediary nodes to provide component isolation for reduced side effects in the ROS-based application's functionality during runtime assessment.\pat{since we talk about the QA team, is this a design guideline (which should be for the developers team) or a testing and verification guideline (which is for the QA team?). }
    
     \subsubsection{Process (HOW)}
     In ROS, the man-in-the-middle (MITM) strategy consists of introducing intermediary ROS nodes between components, in this context the term `components' stands for one or more ROS nodes presenting unique functionality and well-defined interfaces.
     Such intermediary nodes may react by blocking, dropping, modifying, or inspecting the messages passed between components. 
     %In addition, the intermediary node may trigger recovery or rollback mechanisms to restore the system. 
     We identified two means of enacting MITM in ROS, through a proxy design pattern, e.g., ROSRV~\cite{huang:2014}, or through topic remapping, e.g.  ROSMonitoring~\cite{ferrando:2020}. The former works by generating a proxy-based of the ROS Master node which has full control of the nodes and topics during runtime, deploying an intermediary node for message diverting when required. The latter launches an intermediary node and performs topic remapping before execution -- asking for the topic names that should be diverted.

    \subsubsection{Exemplars}~\\
    % \ric{\url{https://arxiv.org/pdf/2305.09933.pdf} \url{https://www.sciencedirect.com/science/article/pii/S0921889022002500?fr=RR-9&ref=pdf_download&rr=81e2f0c37e87abe7}}
    \textbf{Proxy.}    
     ROSRV~\cite{huang:2014} deploys a ROS master node proxy, namely \href{https://github.com/cansuerdogan/ROSRV/tree/master/src/RVMaster}{RVMaster~\faicon{github}}, that acts as a firewall, blocking the access to the ROS master node port. This node, in turn, is responsible for creating MITM nodes (also called monitors) that intercept the messages flowing between nodes in the system. RVMaster instantiates the MITM nodes according to user-provided specifications of access policies, even though it does not require any change to the system under scrutiny. Listing \ref{lst:inerceptors} portrays the |createInterceptors()| method from the RVMaster that enacts MITM monitor nodes by re-subscribing to a new set of topics.
     
\begin{lstlisting}[language=Cpp, label=lst:inerceptors, caption={Creating proxy-based MITM nodes in ROSRV.\vspace{.35cm}}]
void ServerManager::createInterceptors(){

	for (std::map<std::string,std::string>::iterator it=rv::monitor::topicsAndTypes.begin(); it!=rv::monitor::topicsAndTypes.end(); ++it) {
	   string topic = it->first;
		 string datatype = it->second;
		 Monitor *monitor_p = NULL;
		 string monitorname = topic+MONITOR_POSTFIX;
   
	     XmlRpc::XmlRpcValue params, result, payload;
	     params[0] = monitorname;
	     params[1] = topic;
	     params[2] = datatype;
	     string m_uri = "";
	     params[3] = m_uri;

	     //create a xmlrpcmanager-client for each monitor
	     monitor_p = new Monitor(params,rv_ros_host, monitorname);
	     monitorMap[topic] = monitor_p;
	     m_uri = monitor_p->getMonitorXmlRpcUri();
		 params[3] = m_uri;
   		 
	 	 bool f = master::execute("registerSubscriber",params,result,payload,true);

	     //start a new thread with the params
	     boost::thread(boost::bind(&Monitor::monitorThreadFunc, monitor_p));
	     
	     result[0]=1;
      result[1]="Subscribed to ["+topic+"]";
		 XmlRpc::XmlRpcValue pubs_monitor;
		 pubs_monitor[0] = m_uri;
		 result[2] = pubs_monitor;
     
      ROS_INFO("Monitor %s successfully registered a subscriber to topic %s", monitorname.c_str(), topic.c_str());
	  }
\end{lstlisting}

     \textbf{Topic remapping.}
     \href{https://github.com/autonomy-and-verification-uol/ROSMonitoring}{ROSMonitoring~\faicon{github}}~\cite{ferrando:2020} utilizes topic remapping to ensure safety and security in the system by creating intermediary nodes via topic name remapping (\href{http://wiki.ros.org/roslaunch/XML/remap}{roslaunch/remap}). 
     Remapping is a core tool from ROS that enables swapping topic names just before running the application. {\it Remap}, enables inserting an intermediary node between the other two original nodes. Listing \ref{lst:topic_remap} exemplifies the topic remapping-based MITM strategy applied by ROSMonitoring. The code snippet shows that the launch files are incremented with remap statements including the node names, original (`from') topic and new (`to') topic name.

\begin{lstlisting}[language=Python, label={lst:topic_remap}, caption={Topic remapping-based MITM in ROSMonitoring.}]
def instrument_launch_files(nodes):
    ...
    for (name, package, topics) in launch_files[path]:
        if node.get('name') == name and node.get('pkg') == package:
            for topic in topics:
                remap = ET.SubElement(node, 'remap')
                remap.set('from', topic)
                remap.set('to', topic + '_mon')
            break
\end{lstlisting}
    
    %\textbf{Runtime.} \ric{This section is very weak. I hardly understand what it does and how different from Binding Time. I can't explain how do the tools here work.}
    %The \href{https://github.com/ros-tooling/topic_tools}{topic\_tools~\faicon{github}} package is the official ROS throttling tool. It works as a node that subscribes to a particular topic and publishes the incoming messages after performing operations such as type conversion, transformation into another topic and change in the message rate or the bandwidth of the topic, which is also referred to as \emph{throttling}. In addition, using this tool it is possible to drop a certain fraction of incoming messages, which can in turn be used to block a topic completely.  
    %In the task of throttling in particular, there are additional packages developed which are based on the official \textit{topic\_tools} but offer some additional features. For instance, \href{https://github.com/UTNuclearRoboticsPublic/rosthrottle}{rosthrottle~\faicon{github}} allows to programmatically create ROS nodes for the MITM strategy while \href{https://github.com/proboticks/dynamic_topic_tools}{dynamic\_topic\_tool~\faicon{github}} allows to change the throttling message rate and/or bandwidth of the topic at runtime.
    
    \subsubsection{Strengths} The MITM strategy enables freezing of the application at the software level without the normal operation, and rollback in case the test scenarios are prone to side-effects and do not require any change in the code.
    
    \subsubsection{Weaknesses} Placing nodes between computations may cause performance overhead in the system under scrutiny. In addition, erroneous intermediary nodes may affect the functionality of the system, and thus represent a threat to the test's reliability. This guideline does not directly apply to server-based or parameter-based communication. In addition, we understand that isolation can be difficult for robotics. In fact, the two-way interaction between the software and the physical environment makes it impossible to assess the behavior of one in isolation from the other. This can be mitigated, e.g., with model or software-in-the-loop testing approaches.

\section{Guidelines for Quality Assurance through Runtime Verification and Field-Based Testing} \label{sec:test_fulllist}

In this section, we describe twelve guidelines to assist quality assurance teams to attaining confidence on robotic applications developed using the Robot Operating System (ROS). Attaining confidence, in this case, consists of applying runtime verification and field-based testing. 
The Prepare Execution Environment (PE) group contains two guidelines: PE1 to warn about the overhead acceptance criteria, and PE2 to create models for runtime assessment. The Specify (Un)-Desired Behavior group (SDB) contains three guidelines concerning the specification of desired and/or undesired behaviors. SDB1 and SDB2 concern the specification of properties through the use of logic-based languages (SDB1) or Domain Specific Languages (DSLs) (SDB2). SDB3, in turn, focuses on scenario-based specifications of test cases. 
The  Generate Monitors and Test Cases group (MTA) contains two guidelines. MTA1 focuses on how to improve the robustness of the system by performing noise and fault injection. MTA2 discusses how to exploit automation for monitoring and testing, e.g., generation and prioritization of test cases. The System Execution group (SE) contains two guidelines focusing on the importance of using record-and-replay when performing exploratory field tests (SE1) and the importance of headless simulation (without GUI) for optimization and/or automation (SE2). Finally, the Analysis \& Reporting group (AR) contains two guidelines. AR1 focuses on performing postmortem analysis to diagnose non-passing test cases. While AR2 focuses on the use of reliable tooling to manage field data.
            
\subsection{PE1. Understand the overhead acceptance criteria}

            \subsubsection{Context (WHEN)} According to practitioners, performance is among the three most important quality attributes when designing a robotic application in ROS~\cite{malavolta2021mining}. Performance is often important in robotics because many computations performed by robots tend to be data-intensive, e.g., computer vision, planning, and navigation~\cite{malavolta2021mining}. Gaining confidence in robotic applications, then, should not interfere with the nominal performance of the robot under scrutiny. Less (or no) impact on performance is especially desirable when the assurance gathering process interacts with the running system, for instance, in-the-field testing and runtime verification. 
            We name the extra load available for gaining confidence on ROS-based applications as \textit{overhead acceptance criteria}. The overhead acceptance criteria can be allocated to monitoring,  isolation, or maintaining the security of privacy during the runtime assessment session~\cite{bertolino:2021}.
            
            \subsubsection{Reason (WHY)} A rule of thumb says that more observations tend to enable more precise assurance arguments within a limit. %~\cite{shannon1949communication}.
            Observing, however, is never free from side effects, incurring in overhead~\cite{falcone:2021}. Therefore, the quality assurance team must contrast the precision of the assurance arguments against overhead introduced by the observation medium. The overhead acceptance criteria are the basis for deciding the runtime assurance strategy. 
            
            \subsubsection{Suggestion (WHAT)} %Before committing to a runtime assurance strategy, the QA team should understand the overhead acceptance criteria by means of monitoring overhead, isolation overhead, and security and privacy maintenance overhead.
            The use of runtime verification or field-based techniques might add computation overhead.
            The QA team should understand how much overhead is acceptable; this is important to decide on a test strategy that will not severely impact the performance of the running system. Such overhead may be due to monitoring with ros\_tracing (git: ros2/ros2\_tracing), component isolation, or security and privacy maintenance overhead with ROSploit (git: seanrivera/rosploit).
            %For example, by means of monitoring overhead, isolation overhead, and security and privacy maintenance overhead.
            
            \subsubsection{Process (HOW)} Typically, understanding the overhead acceptance criteria follows from contrasting the required performance for delivering the required service, aka nominal performance (e.g., time to reaction, latency, speed), against available resources (e.g., computing power). The QA team may use off-the-shelf ROS tooling, like ApexAI/Performance$\_$test~\href{https://gitlab.com/ApexAI/performance_test}{\faicon{gitlab}}, to understand the nominal performance of the ROS-based application. The difference between nominal performance and expected performance may be allocated to the overhead acceptance criteria. If the nominal performance is close enough to the expected performance, there is not enough space for implementing runtime assurance techniques. We categorise three types of overhead that may affect the runtime assurance process: Runtime Monitoring~\cite{ferrando:2020,BEDARD2023104361}, Isolation overhead~\cite{lahami2016safe,silva2022self}, and Security and Privacy overhead~\cite{rivera:2021,breiling2017secure}.
    
            \subsubsection{Exemplars}~\\ 
            \textbf{Monitoring overhead} is all extra load put on the system-under-test due to gathering, interpreting, and elaborating data about the execution. For example, ROSMonitoring (autonomy-and-verification-uol/ROSMonitoring~\href{https://github.com/autonomy-and-verification-uol/ROSMonitoring}{\faicon{github}})~\cite{ferrando:2020} determines the monitoring overhead by calculating the delay introduced in the message delivery time between ROS nodes. The authors analyse the overhead by varying the size of the system under monitoring, message passing frequency, and number of monitor nodes. However, their overhead analysis is not transparent with respect to gathering, interpreting or elaborating on data, the analysis looks at the monitoring overhead as a black box. Another example is ros2\_tracing (ros2/ros2$\_$tracing ~\href{https://github.com/ros2/ros2_tracing}{\faicon{github}})~\cite{BEDARD2023104361} that provides a tool for tracing ROS2 systems with low latency overhead. The authors measure monitoring overhead by collecting the time between publishing a message and when it is handled by the subscription callback. In short, monitoring and tracing tools add some overhead that typically affects the message passing latency, the QA team must understand and define a precise time allowance to this overhead.\\
            \textbf{Isolation overhead} is all extra load put on the system-under-test for guaranteeing that the runtime assessment will not interfere with the normal operation or produce undesired side effects. As an example, Lahami M. et al.~\cite{lahami2016safe} propose a safe and resource-aware approach to test dynamic and distributed systems. % (similar to ROS-based systems).
            Safe by employing testing isolation techniques such as BIT-based, tagging-based, aspect-based, cloning-based, and blocking-based.
            Resource aware by setting resource monitors such as processor load, main memory, and network bandwidth. 
            The authors show that the overall overhead is relatively low and tolerable, mainly if dynamic adaptations are not commonly requested. However, there is no fine-grained evaluation of the overhead introduced by isolation techniques. In fact, isolation overhead is rarely reported~\cite{silva2022self}.\\
            \textbf{Security and Privacy overhead} is all extra load put on the system-under-test for maintaining security and privacy constraints while testing. For example, ROS-Immunity is a security tool for preventing ROS-based applications from malicious attackers. Rivera S. et al.~\cite{rivera:2021}, determines overhead for maintaining the ROS-based system secure, while operating, in terms of power consumption (in Watts) by comparing the power draw of the system with and without their tool. From another stance,  Breiling B. et al~\cite{breiling2017secure} present a secure communication channel to enable communication between ROS nodes using protocols such as Transport Layer Security (TLS) and Datagram Transport Layer Security (DTLS) per each ROS topic in the application. The protocols follow three steps: an initial handshake with mutual authentication, using symmetric encryption (AES-256), and using Message Authentication Codes (MAC) for data integrity. Importantly, they evaluate the overhead introduced for each step, totalling in a few percentage points (2\%-5\%) of increase in average CPU load.

            \subsubsection{Strengths} Understanding the overhead acceptance criteria in advance may avoid unexpected interruptions in the ROS application functionality due to runtime quality assessment procedures. For example, when testing procedures are mistakenly scheduled whenever the ROS-based application is operating under a high load. Learning about the overhead in advance criteria may also ask for re-design due to a lack of verifiability during runtime. For example, when the nominal performance of the ROS system is close to the expected performance, in value.
            
            \subsubsection{Weaknesses} Although there is tooling to support the assessment of the overhead acceptance criteria, the process for understanding involves executing the system, collecting performance data and analysis. This may conflict with time-to-market requirements, asking for further negotiation with the business goals of the ROS-based system.

\subsection{PE2. Create models for runtime assessment}\label{sec:PE2} 

            \subsubsection{Context (WHEN)} %ROS applications typically interact with the physical environment and other third-party software modules. 
            Gaining confidence in the running systems can be costly due to the need for isolation from side effects, preservation of security and safety, controllability, and observability~\cite{bertolino:2021}. One way to address this issue is through the use of model-based runtime assessment, which can help to manage complexity and ensure the safe operation of ROS-based applications~\cite{schlegel2009robotic}. Models can be used to define safety criteria, create digital twins of the system and its environment, and ensure adequate test coverage. This guideline discusses creating models for managing the complexity of runtime assessment in ROS.
            
            \subsubsection{Reason (WHY)} 
            Modeling is essential for efficient and effective testing of ROS-based systems in the field. ROS-based systems lack a built-in system representation, making it difficult to identify and address bugs without costly calibration of sensors and actuators~\cite{kirchhof2020model,guerrero:2021,lewis:2022}. By incorporating models, such as those used in low-fidelity simulation, the testers can reveal the same bugs found in real-world navigation~\cite{sotiropoulos2017can}. Implementing models in runtime assessment of ROS-based systems can save costs and improve the overall performance of the tests.
            
            \subsubsection{Suggestion (WHAT)} %To manage the complexity of runtime assessment in ROS, the QA team might create and exploit suitable models of the system itself, models of the environment and metamodels.
            The QA team might create and exploit models of the system and/or of its environment (a sort of digital twin) for runtime assessment, predictive maintenance, checking alternatives, and so on. For example, they can create a digital twin of the system by using CPSAML (me-big-tuwien-ac-at/cpsaml), or formal tools such as UPPAAL combined with UPPAALTron (doi: 10.1109/ECMR.2015.7324210). In addition, the QA team may use ROS metamodels (ipa-nhg/ros-model) to facilitate the use of tools and graphical plug-ins for reverse engineering models from ROS code.

            \subsubsection{Process (HOW)} Models can be used to create useful representations of the system's components for runtime assessment of ROS-based applications, such representations include (i) models of the system itself, (ii) models of the environment and (iii) metamodels.(i) Models of the system itself consider digital twins of the system or part of the system~\cite{saavedra2022ros,fend2022cpsaml}. (ii) Models of the environment may be carried out in tools for formal verification, e.g., UPPAAL~\cite{ernits2015model,larsen2005testing}. (iii) Metamodels rely on the Eclipse Ecore technology to encoding rules for modeling, generating and introspecting ROS-based systems~\cite{garcia2019boot1,hammoudeh2021} 
            %safety models, digital twins of the system, models of the environment, and ROS metamodels for reverse engineering and tooling. These models can come in various forms, such as automata-based models, UML models, 3D models (use siemens/ros-sharp~\href{https://github.com/siemens/ros-sharp}{\faicon{github}}), mockups in the host language, and Eclipse EMF models. 

            \subsubsection{Exemplars} ~\\
            \textbf{Models of the system itself}.
            Saavedra Sueldo C. et al.~\cite{saavedra2022ros} proposes an architecture for integrating digital twins (DTs) on production systems using ROS. The paper argues that digital twins should be used as the central component for the formulation of autonomous decision-making systems due to their static nature. In order to do this, in their online repository (INTELYMEC/ROS$\_$Tecnomatix ~\href{https://github.com/INTELYMEC/ROS_Tecnomatix}{\faicon{github}})  the authors provide a ROS node (named plant$\_$simulation$\_$node) that performs the same operations (e.g., decision using a method of reinforcement learning and a material handling procedure) of its counter-part, but in a controlled environment. The simulation node can be understood as a mock or model of self.  In a similar direction, Fend A. and Bork D.~\cite{fend2022cpsaml} suggest model-driven runtime monitoring based on digital twins for ROS-based applications, namely CPSA$_{ML}$(me-big-tuwien-ac-at/cpsaml~\href{https://github.com/me-big-tuwien-ac-at/cpsaml}{\faicon{github}}). CPSA$_{ML}$ generates local DT components that are executed as ROS nodes. The DT component holds the state of the DT entity; in other words, it provides a model of the execution life-cycle of its counterpart. Ultimately, the model of the system can be used for reasoning during testing and runtime verification. \\ 
            \textbf{Models of the environment}. The test setup described in Ernits et al.~\cite{ernits2015model} uses UPPAAL Tron~\cite{larsen2005testing} as the primary test execution engine. First, the QA team should model, in UPPAAL, (i) an implementation model of the system under test and (ii) a topological map of the environment. Second, the QA team integrates an adapter, provided by Ernits et al.~\cite{ernits2015model}, which is responsible for translating messages between the environment model and the appropriate topics in ROS, acting as the interface between the ROS-based system under test and the UPPAAL Tron model of the environment. Finally, the interaction between the implementation model (i) and the environment model (ii) is monitored during system execution and afterwards, the equivalence between the measured outcomes from the running system and the outcomes from the model is checked. 
            %\gena{It seems rather limited the number of works in this particular issue. Does this indicate sth like: too novel? too costly? etc...} 
            The operating environment, however, is typically prone to uncertainty which makes modeling the environment a costly activity.   \\
            \textbf{Metamodels}. One of the most notable works using models as a foundation for software development with ROS is the series on Bootstrapping MDE Development from ROS Manual Code~\cite{garcia2019boot1,hammoudeh2021} by Hammoudeh Garcia N. In the repository (ipa-nhg/ros-model~\href{https://github.com/ipa-nhg/ros-model}{\faicon{github}}), a set of metamodels defined as Ecore models are provided to facilitate the use of tools and graphical plug-ins for creating models from ROS code, composing and validating model compositions, auto generating deployment artifacts, and checking the use of standard specifications. The repository also includes tutorials on reverse engineering from ROS code to models, creating a model using introspection at runtime, and generating ROS code from models.

            \subsubsection{Strengths} By using models for field-based testing, it is possible to reveal bugs in a safe and cost-effective way, without the need for costly and risky test campaigns in the field; It also allows for flexibly choosing the model representation, and the level of detail of the model, according to the needs of the system, the test scenarios, and the available resources. Models can be reused in different testing scenarios, and across different system components, reducing the effort and time required for testing.

            \subsubsection{Weaknesses} {\color{blue} Large and complex robotics systems may impair the creation and maintenance of runtime models}\footnote{Added after follow-up questionnaire on April 14th.}. Models need to be updated and maintained as the system evolves, which can be a costly and time-consuming task. In addition, modeling can be prone to errors and inaccuracies, which can affect the quality of the testing results. Models are domain dependent and may not be easily transferrable between domains such as healthcare domain, automotive, or aerial domains. %\todo{read comments and add discussion about knowledge transfer and taxonomy w.r.t models} %\gena{Should you also mention the gaps in the state-of-the-art regarding, for example, the need for more comprehensive domain application for those models? Or even evidence that practitioners should/may adopt?} 

\subsection{SDB1. Property specification using a logic-based language}\label{sec:SDB1} %ROS-based formal description language}.
    
     \subsubsection{Context (WHEN)} %ROS applications typically interact with the physical environment and other third-party software modules. 
            Robotics systems are complex, inherently hybrid systems that combine hardware and software components and whose behaviour is often dictated by close safety, legal, and ethical considerations~\cite{luckcuck:2019}. Furthermore, given the increasingly frequent deployment of ROS-based systems in safety-critical environments coupled with their dependence on complex decision-making and sophisticated control systems, it becomes necessary to find a form of verification that can reliably assess the correctness of these systems. This guideline discusses the use of formal and logic-based languages for specifying properties for runtime verification and/or field-based testing.

            % \textbf{[Reason]} santos:2021
            \subsubsection{Reason (WHY)}
            A logic-based language for verification and/or testing allows specifying properties that describe observable actions, outputs, how they relate to each other and when they should manifest~\cite{santos2021safety}. The behaviour is often described using temporal logic, which enables the specification of desired or undesired 
            %. 
            %The use of a verification tool with a logic-based language guarantees that the tool is able to inspect 
            interactions amongst multiple components (ROS nodes) regardless of the complexity of the system. To simplify the specification of properties in temporal logic, some of the tools refer to existent property specification patterns~\cite{autili:2015}, i.e., a collection of existing known recurrent patterns for the specification of temporal properties. Specification patterns also enable the properties formulation in English thanks to a bidirectional mapping from various temporal logics to a  structured English grammar.  %, and in a manner that is robust to system adaptation and(or) evolution. Furthermore, the properties defined using these verification tools generally align with the catalogue of specification patterns \cite{menghi:2021}, which provides additional standardization and usability to the validation system. 
            %\pat{Note to myself: add something about the patterns}
            
            \subsubsection{Suggestion (WHAT)} %The QA team should be prepared to specify properties using a logic-based language, as often required by verification tools; instruments, like specification patterns, might facilitate the error-prone specification process and to make the specification accessible to people lacking expertise in logic.
            The QA team should be prepared to specify properties using unambiguous and precise languages like logic-based languages, as often required by verification tools. User-friendly instruments, like specification patterns \url{http://ps-patterns.wikidot.com/}, might facilitate the error-prone specification process and make the specification accessible to people lacking expertise in logic. For example, HAROS (git: git-afsantos/haros) uses a logic-based language called HPL for property specification that is used to synthesize runtime monitors for testing and verification.
            
            \subsubsection{Process (HOW)} 
            There are several choices of tools that use logic-based languages for properties specification~\cite{santos:2021,lesire:2019,hu:2019,nickovicrtamt,aldegheri2021containerized}. These tools allow for safety, security, and liveness analyses.
            The formal specification languages for ROS-based systems should provide references to individual resources (e.g. topics) and message contents as well as temporal operators and relations in addition to real-time behaviour specifications.%\ric{Tony, we must cite here all exemplars in the exemplars section. This explanation is missing: \cite{aldegheri2021containerized,nickovicrtamt}. Also, I don't see \cite{lesire:2019} and \cite{hu:2019} in the exemplars. Should we include them there or remove them from here? Maybe we don't need to describe exemplars from them directly there.}

            \subsubsection{Exemplars}~\\ 
            The identified tools make use of various types of temporal logic.  \\
\noindent \textbf{Linear Temporal Logic (LTL).} %Several of the reviewed tools derive their language semantics from Temporal Logic. \tony{Want to consult with Patrizio the name and definition of the section.} 
            %An instance of  logic-based runtime verification is shown in~\cite{aldegheri2021containerized}. In this work, the authors 
            The work in~\cite{aldegheri2021containerized} proposes a novel architecture, for assertion-based verification by using monitors synthesized automatically from Linear Temporal Logic (LTL) assertions. Then, the monitors are encapsulated into plug-and-play ROS nodes and docker containerization is used to improve system portability. As an example, Listing~\ref{lst:LTL} shows an LTL assertion to check if a robot arrives at a position $<x_2,y_2>$ before a certain timeout.
\begin{lstlisting}[language={LOGIC}, caption={LTL assertion to check if a robot reaches a desired position}, label={lst:LTL}, commentstyle=\color{dkgreen}]
always((robot x1 = x1 && robot y1 = y1  && newGoal) 
implies 
(currentTime < timeOut U robot x2 = x2 && robot y2 = y2))
\end{lstlisting}

             \noindent \textbf{Signal Temporal Logic (STL).} Signal-temporal logic is a special case of MTL where properties are defined over signals. They enable real-time reasoning and constraint specification. In \cite{nickovicrtamt,yamaguchi2023rtamt}, Signal Temporal Logic (STL) is used to describe Cyber-Physical Systems (CPS) properties. The approach introduces the novel quality of \textit{robustness semantics}, which implies the system's ability to measure how far is an observed behaviour from satisfying or violating a specification. %Moreover, Nickovic et al. provide an interface to RTAMT (Real-Time  Monitoring Tool) specific to ROS, namely \href{https://github.com/nickovic/rtamt4ros}{rtamt4ros\faicon{github}}~\cite{nickovicrtamt}. 
            Concretely, the developed tool was \textbf{rmtat}~\href{https://github.com/nickovic/rtamt}{\faicon{github}}, which was later augmented to support integration with ROS-based systems with \textbf{rtamt4ros}~\href{https://github.com/nickovic/rtamt4ros}{\faicon{github}}. \\
            \noindent \textbf{Metric Temporal Logic (MTL).} Some runtime verification tools add the ability to handle real-time specifications since the reaction time can have a strong influence on the success or failure of the robot's mission.            
            %given that, for example, although a response to a stimulus 1 second after and 100 milliseconds after both occur \textit{eventually}, the time difference could result in the success or failure of the robot mission. 
            Taking this aspect into consideration, the RV tools described in~\cite{santos:2021,hu:2019} use Metric Temporal Logic. On the other hand, \cite{lesire:2019} addresses it by combining Past-Time LTL to express complex formulas with timed constraints on the evaluation of these formulas. Hu et al. design their robot monitoring specification language based on Discrete Time-MTL (DT-MTL)s~\cite{hu:2019}. The language's syntax embeds a time interval in the traditional MTL notation. Their approach uses the system's periodic nature to discretize the real-time property and replace the real number in time constraints with the number of CPU clock cycles.\\
            \noindent \textbf{TCTL.} Timed automata is one of the most widely used formal models to specify and verify real-time systems. Rodrigues A. et al. specify timing constraints using Timed Computational Tree Logic (TCTL) to encoding the requirements of a safety-critical healthcare monitoring system in ROS\href{https://github.com/rdinizcal/SEAMS18/tree/master/uppaal}{seams18/uppaal~\faicon{github}}~\cite{Rodrigues2018}. Halder et al. specify UPPAAL models over ROS applications by performing manual code analysis. This phase requires the extraction of ROS code parameters that affect the desired properties of ROS-based robotic applications, including the publishing rate, the subscriber's spin rate to process callbacks, the time to transmit messages over channels, and the time to process callbacks. Properties are specified over queue overflow constraints~\cite{halder2017formal}. \\
            \noindent \textbf{Patterns-based specification.}
            In \cite{santos:2021}, the authors introduce HAROS, which is a framework for quality assurance of ROS-based code. The use of the formal language HPL ensures that after entering a state of high priority (where the messages in the topic \textit{'/state'} have \textit{data} greater than $0$), the system should remain in that state for, at least, one second. This can be accomplished through the following property definition:
            {\footnotesize \texttt{{"\textbf{globally}: /state \{data $>  0$\} \textbf{forbids} /state \{not data $>  0$\} \textbf{within} 1000 ms"}}}. As can be seen, the property specification makes use of specification patterns, similar to the {\em absence} pattern with a time constraint~\cite{autili:2015}. Recently, other sets of patterns specific to robotics have been defined~\cite{menghi:2021,patterns2022}; even though they have been conceived for mission specification, they could be profitably used for verification and (scenario-based) testing.
    
    \subsubsection{Strengths} Using logic-based languages to specifying properties offers a standardized approach to validation in compliance with well-adopted specification pattern.

    \subsubsection{Weaknesses} It is noted that the properties' expressiveness is often limited by the description language meaning that diffent languages and tool sets may enable specific property specifications or not.
    
\subsection{SDB2. Use Domain Specific Languages to Specify Properties}\label{sec:SDB2} %Use a ROS-based Domain Specific Language for specyfing the properties.} 

    \subsubsection{Context (WHEN)} 
    To address the safety challenge, one option is defining a clearly specified and isolated layer, which is declared separately from the main program and that can express the functional safety-critical concerns in terms of externally observable properties of the software~\cite{adam2016rule}. This guideline discusses the use of a Domain Specific Language to define the properties of the system.
 
    \subsubsection{Reason (WHY)}
    As a more informal, code-like alternative, the QA team has the choice of utilizing a Runtime Verification tool that has a built-in ROS-tailored language and allows the quality assurance team to specify and validate the correct behaviour of the system. 
    
    \subsubsection{Suggestion (WHAT)} %The QA team may use a verification tool that allows the definition of properties using a DSL to facilitate the verification and/or testing activities.
    In complement to logic-based instruments, the QA team may opt to use verification tools that allow code-like specifications of properties to simplify the definition of the desired behavior. For example, ROSMonitoring (git: autonomy-and-verification-uol/ROSMonitoring) allows for code-like specifications of properties in a domain specific language (DSL) targeted to the properties such as writing assertions over the robot's position using if-else constructs.     
    
    \subsubsection{Process (HOW)}
    The works in~\cite{adam2016rule,ferrando:2020,huang:2014} describe DSLs for specifying properties.
    The properties described with the DSL are checked mainly by intercepting the messages from relevant services and topics from the ROS system. It is important to consider the nature of the properties that should be specified and the expressiveness of the DSL. These DSLs give often the possibility to specify actions that should be performed in reaction to a violation of a safety property. It is important that the QA team chooses, customizes or conceives the DSL that best suits the specific needs. 

    \subsubsection{Exemplars}~\\ 
    %\ugh{Understand if we write this here: \cite{morse2023framework}}    
    The runtime verification tools described in~\cite{ferrando:2020,huang:2014} are based on a DSL that allows collecting the information from the different software components (ROS nodes) at a given moment in time and perform a corresponding action if one or more of the predefined rules are broken. 
    In \cite{huang:2014}, the authors define ROSRV. Listing~\ref{lst:dsl-rosrv} shows the definition of a condition for which the system will be monitoring and the corresponding action to be taken in case a violation occurs. 

\begin{lstlisting}[language={LOGIC}, caption={Example of position and velocity property specification in ROSRV\vspace{.35cm}}, label={lst:dsl-rosrv}]
event moveOrStop(double lx, double ly, double lz) 
/landshark_control/base_velocity 
geometry_msgs/TwistStamped 
'{twist:{linear:{x:lx,y:ly,z:lz}}}'
{
  if( posx > 9 ) {
    if(vectory * lx < 0) {
      ROS_WARN("Position not allowed");
      return;
    }
  }
}
\end{lstlisting}

    In ROSRV, the event definition structure is as follows. First, the keyword event must be followed by the event name and the parameters that need to be provided to the method. Consequently, one must state the topic name, data type and the mapping from the topic information to the method parameters. Such structure is shown in Listing~\ref{lst:dsl-rosrv}.

    In \cite{adam2016rule}, the property definition DSL (namely RuBaSS) allows incorporating time into the rule definition. For example, one can describe a safety property as {\footnotesize \texttt{"max\_speed\_exceeded: linear\_speed $>$ max\_speed for 2 sec;"}}  where the \textit{linear\_speed} and \textit{max\_speed} values are extracted from messages published in corresponding topics. Consequently, this property checks whether the comparison holds true for 2 seconds using the DSL defined by the authors.
    
    \subsubsection{Strengths} The use of Domain Specific Languages for specifying properties brings a programmer-friendly interface for runtime validation. Moreover, it promotes the definition of well-structured and standardized approaches.

    \subsubsection{Weaknesses} On the negative side, the expressiveness of properties is limited by the DSL used.

\subsection{SDB3. Use languages and tools to scenario-based specification of test cases}\label{sec:SDB3}

    \subsubsection{Context (WHEN)} Scenario specification allows the QA team to test robots on credible and complex activities since it defines the course of a robotic mission~\cite{afzal:2020}. 
    Gathering confidence in autonomous systems through so-called verified scenarios is a cornerstone of simulation testing~\cite{luckcuck:2019}. However, designing test cases in the form of scenarios implicitly requires accounting for possible variations and conditions. This makes scenario-based testing a challenging task and often deemed infeasible. In addition, unexpected scenarios frequently underlie failures in robotic systems~\cite{afzal:2020}. Therefore, it is important to consider real-world data during scenario generation since it permits to focus on a range of scenarios that can be unexpected during the design phase~\cite{bertolino:2021}.

    \subsubsection{Reason (WHY)} Scenario-based test case generation is a powerful approach to verify ROS-based applications because it allows for the systematic exploration of different situations and conditions that the robotic system may encounter in the real world. By defining scenarios, the testing team can ensure that the application behaves correctly under a wide range of circumstances, including both expected and unexpected events.

    \subsubsection{Suggestion (WHAT)} %To enable a systematic exploration of real-world situations and conditions, the QA team might integrate scenario specification languages and tools to ROS-based applications.
    The QA team might integrate scenario specification languages and tools to enable a systematic exploration of real-world situations and conditions for ROS-based applications. For example, Geoscenario (git: rodrigoqueiroz/geoscenarioserver) uses behavior trees to program dynamic interactions between the system-under-test and other vehicles in the scenario. In addition, SCENIC (git: BerkeleyLearnVerify/Scenic) is a probability-based programming language that enables the specification of rare events in environment models that are used to generate test cases for vehicles running on the CARLA simulator (git: carla-simulator/carla) that may be further integrated to testing ROS-based systems.

    \subsubsection{Process (HOW)} To implement scenario-based specifications for testing ROS-based applications we recommend describing technology enablers and motivating use cases. Technology enablers, in this case, list a set of languages that assist the design of scenarios for testing ROS-based applications. The technology-enablers vary with respect to human-vehicle behavioral description~\cite{queiroz2022driver}, to probability-based programming of scenarios~\cite{fremont2022scenic}, and integrating graphical simulation with Simulink-based control design and ROS~\cite{xu2022sil}. From the point-of-view of use cases, scenario specification may turn useful to perception monitoring ~\cite{balakrishnan:2021}, validating multi-layered control strategies ~\cite{duan2021implementing}, and pedestrian simulation scenarios~\cite{liu:2017}.

    \subsubsection{Exemplars}~\\ 
    \textbf{Technology-enablers:}
    \href{https://github.com/rodrigoqueiroz/geoscenarioserver}{GeoScenario~\faicon{github}}~\cite{queiroz2022driver} proposes using a behavior tree-based DSL to describe autonomous human-vehicle models for scenario-based testing. The toolset advocates for scenario specifications that reflect dynamic interactions between humans and the subject system in real traffic conditions. Therefore, behavior trees are used as a fundamental control-flow strategy. GeoScenario interfaces with a simulation layer where LIDAR and camera capture data from the vehicle controller implemented at ROS-level. Listing \ref{lst:geoscenario} showcases an implementation of one of the agent's behavior in a pre-crash scenario from NHTSA. The vehicle changes the lane to the left, then continues driving using another drive\_tree implementation. The operator '?' stands for fallback operation, '-\>' is sequential, 'condition' evaluates to a Boolean value, and 'maneuver' executes a task.

\begin{lstlisting}[language={BT}, caption={Lane change human-vehicle implementation in Geoscenario.\vspace{.35cm}}, label={lst:geoscenario}]
behaviortree LaneChange:
  ?
    ->
      condition c_trigger(sim_time (tmin=4))
      ->
        condition c_reach(gap(target_lane=Left,range=5,repeat=False))
        maneuver cutin(MCutInConfig(target_lane=Left,delta_s=(5,-3,0)))
    subtree drive_tree(m_vel_keep=MVelKeepConfig(vel=MP(14.0,10,6)))
\end{lstlisting}
    
    \href{https://github.com/BerkeleyLearnVerify/Scenic}{SCENIC~\faicon{github}}~\cite{fremont2022scenic}, a probability-based programming language, argues for the specification of rare events in environment models for autonomous vehicles and robots for testing purposes. The language relies on the specification of \textit{scenarios}, i.e., configurations of physical objects and agents, and how they change over time. In combination with CARLA~\cite{dosovitskiy2017carla}, SCENIC can be used to specify scenarios for ROS-based simulation test scenarios. For example, departing from a Metric Temporal Logic (MTL) safety specification, SCENIC generates (with VERIFAI~\cite{tommaso2019verifai}) 2000 scenarios for a vehicle performing a right turn at an intersection, yielding to the crossing traffic.

%     \begin{lstlisting}[language={LOGIC}, caption={Scenario specification example using SCENIC}, label={lst:SCENIC}]
% "scenario": {
%     "location": [1015.6, 736.8],
%     "time": [22, null],
%     "weather": "RAIN",
%     "vehicle": "voltic",
%     "drivingMode": -1
% }
%     \end{lstlisting}

    Supporting Software-In-the-Loop (SIL) simulation testing, Xu C., et al.~\cite{xu2022sil}, introduces a platform that unites PreScan~\cite{tideman2010scenario}, MATLAB/Simulink~\cite{simulink}, and ROS. The three-layered platform enables virtual sensors and scenarios designed in PreScan, control design in MATLAB/Simulink, and environment perception, planning and control execution at ROS-level. The proposed stack features graphical scenario specification including sensor simulation and may be used for mobile robotics with a focus on self-driving simulation testing.\\ 
%    
    %\begin{itemize}
        %\item SIL simulation -- \href{https://ieeexplore.ieee.org/abstract/document/9970607}{https://ieeexplore.ieee.org/abstract/document/9970607}
        %\item \href{https://ieeexplore.ieee.org/stamp/stamp.jsp?tp=&arnumber=8244165}{https://ieeexplore.ieee.org/stamp/stamp.jsp?tp=\&arnumber=8244165}
        %\item \href{https://link.springer.com/chapter/10.1007/978-981-15-5580-0_27}{https://link.springer.com/chapter/10.1007/978-981-15-5580-0\_27}
        %\item \href{https://ieeexplore.ieee.org/stamp/stamp.jsp?tp=&arnumber=9304609}{https://ieeexplore.ieee.org/stamp/stamp.jsp?tp=\&arnumber=9304609}
        %\item DSL to scenario specification:
        %\begin{itemize}
        %    \item Geoscenario\href{https://arxiv.org/pdf/2205.02911.pdf}{https://arxiv.org/pdf/2205.02911.pdf}
        %\end{itemize}
    %\end{itemize}
%
    \textbf{Use Cases:} The work in \cite{balakrishnan:2021} integrates \href{https://github.com/CPS-VIDA/PerceMon.git}{PerceMon~\faicon{github}}, a tool for monitoring spatio-temporal specifications for perception systems, with the CARLA simulator (integrated with ROS), and, in cohort with the OpenSCENARIO specification format defines a set of high-level scenarios for their experimentation setting. Their experimental scenario features sunlight exposure, cyclists crossing or poorly occluded pedestrians, and rendering corner case test fixtures. Similarly, \cite{duan2021implementing} utilizes a ROS-CoppeliaSim~\cite{coppelia} integration to validate their three-layered control decoupling strategy for lateral and longitudinal motion. The tool permits defining motion constraints to the mechanical joint points of the high-precision vehicle model, which forms a front-wheel steering and rear-wheel drive smart car model powered by Ackerman steering. \cite{liu:2017} uses \href{https://github.com/srl-freiburg/pedsim_ros}{pedsim\_ros~\faicon{github}}, a pedestrian simulator tool that relies on XML scene specification, for example Listing \ref{lst:pedsim_ros}.
            
\begin{lstlisting}[language={XML}, caption={Corridor scenario specification with pedsim\_ros~\href{https://github.com/srl-freiburg/pedsim_ros/blob/master/pedsim_simulator/scenarios/corridor.xml}{(Link to source).}\vspace{.35cm}}, label={lst:pedsim_ros}]
<?xml version="1.0" encoding="UTF-8"?>
<scenario>
  <!--Obstacles-->
  <obstacle x1="-0.5" y1="-0.5" x2="29.5" y2="-0.5"/>
  <obstacle x1="-0.5" y1="-0.5" x2="-0.5" y2="14.5"/>
  <obstacle x1="-0.5" y1="14.5" x2="29.5" y2="14.5"/>
  <obstacle x1="29.5" y1="-0.5" x2="29.5" y2="14.5"/>

  <waypoint id="east" x="5" y="5" r="2" b="1"/>
  <!-- Sink -->
  <waypoint id="west" x="25" y="5" r="2" b="2"/>

  <waypoint id="robot_goal" x="22" y="27" r="2"/>
  <waypoint id="robot_start" x="4" y="4" r="2"/>

  <agent x="4" y="4" n="1" dx="0" dy="0" type="2">
    <addwaypoint id="robot_start"/>
    <addwaypoint id="robot_goal"/>
  </agent>

  <!--AgentClusters-->
  <source x="2" y="5" n="8" dx="3" dy="5" type="0">
    <addwaypoint id="east"/>
    <addwaypoint id="west"/>
  </source>
</scenario>
\end{lstlisting}
    
    \subsubsection{Strengths} Scenario-based testing provides a systematic and comprehensive approach to verify ROS-based applications under various conditions. The integration of scenarios with ROS-compatible simulation environments allows for realistic and repeatable testing.
    
    \subsubsection{Weaknesses} The exemplars provided are primarily focused on the automotive domain, which may limit the generalizability of the guideline to other robotic application domains.

\subsection{MTA1. Improve the robustness of the system by performing noise and fault injection }\label{sec:GMTC1}

    \subsubsection{Context (WHEN)} 
    When testing a robotic system, the QA team needs to gain confidence that it will behave safely when faced with unexpected inputs~\cite{hutchison2018}. Techniques such as Fault Injection (FI) and Noise Injection (NI) can aid the QA team in identifying weaknesses, evaluating the resilience of the system as well as measuring its performance under stress. The deliberate introduction of faults such as hardware failures, network interruptions, software errors and signal alterations, can help assess how well the system recovers from these issues. In addition, fault injection is the central tool of a technique called Fault Based Testing, in which the generated test cases address potential faults that can be foreseen at design time\cite{bertolino:2021}.

    \subsubsection{Reason (WHY)} Testing techniques based on fault injection and noise injection aid in increasing the overall reliability of the system under testing.
    
    \subsubsection{Suggestion (WHAT)}
    %To gain confidence that a robotic system will behave safely when faced with unexpected inputs, the QA team can use tools that generate perturbations or inject faults within the testing approach.
    The QA team can use tools that generate noise or inject faults to gain confidence that a robotic system will behave safely when faced with unexpected situations. For instance, RoboFuzz (git: sslab-gatech/RoboFuzz) enables the generation of faults (in ROS 2 applications) through message mutation with three intents: violation of physical laws, violation of user-specified properties, and cyber-physical discrepancies. Moreover, RosPenTo (git: jr-robotics/ROSPenTo) enables security assessment by (un-) registering publishers or subscribers, isolating nodes or services, and injecting false data in the messages in ROS 1 applications.
    
    \subsubsection{Process (HOW)}
    Fault injection is a testing technique to evaluate the robustness of a system that consists of intentionally introducing faults, failures and errors into the software system. The fault injection can occur at various levels, these generally are defined as the software, the hardware and the network layer. In the software layer, for instance, typical operations include the modification of variables and the manipulation of input data.
    Noise injection, instead, refers to introducing noise or interference into a system with the aim of improving the system's resilience. 
    Several tools have been developed in recent years to apply these concepts in the ROS domain, either based on noise injection \href{https://github.com/aliasrobotics/ros1_fuzzer}{ ros1\_fuzzer~\faicon{github}}
    ros2\_fuzzer~\href{https://github.com/aliasrobotics/ros2_fuzzer}{\faicon{github}}~\cite{10.1145/3540250.3549164} or fault injection~\cite{yayan2023,hsiao2021mavfi} \textit{ROS Fault Injection Toolkit}\href{https://github.com/jpdias/ros_fault_inj_toolkit}{~\faicon{github}} \textit{camfitool}\href{http://wiki.ros.org/camfitool}.

    \subsubsection{Exemplars}~\\
    \textbf{Noise Injection:} With the goal of effectively stressing a data-driven ROS system, Seulbae Kim et al.~\cite{10.1145/3540250.3549164} implemented \href{https://github.com/sslab-gatech/RoboFuzz}{RoboFuzz~\faicon{github}}, which is based on a data type-aware mutation technique aimed at finding correctness bugs in the system. RoboFuzz takes a target system and a test strategy as input and outputs the report of found bugs after performing a fuzzing technique based on message mutation.
    In addition, RosPenTo~\cite{dieber2020penetration} (\href{https://github.com/jr-robotics/ROSPenTo}{jr-robotics/ROSPenTo~\faicon{github}})  provides the operations of unregistering and registering publishers/subscribers, isolating nodes and services, and injecting false data in messages. As an example, the authors show how to use the tool to isolate the safety monitor node and to inject fault data in a robotic operation in such a way that the robot may harm humans~\cite{dieber2020penetration}. \\
    % \ric{Scenic has a notion of adding noise to test scenarios, look at: \href{https://www2.eecs.berkeley.edu/Pubs/TechRpts/2018/EECS-2018-8.pdf}{technical report}}
    \textbf{Fault Injection:} Targeting the inclusion of Fault Injection in the system, the \href{https://github.com/inomuh/imfit}{imfit~\faicon{github}} tool, which is based on applying mutation testing to relevant files with the ROS source code, is of great value~\cite{yayan2023}.
    The tool allows the user to create fault injection plans and select the operating conditions for the mutation process. Furthermore, fault metrics and diagrams can be obtained afterwards to analyze the system's response.
   
    In addition, \href{https://github.com/jpdias/ros_fault_inj_toolkit}{ROS Fault Injection Toolkit~\faicon{github}} is a tool that aims to test the reliability and fault-tolerance of a ROS-based system while allowing for user-controlled fault injection, targeting especially the domain of image processing for autonomous driving. Similarly, \href{http://wiki.ros.org/camfitool}{camfitool} is an official ROS tool which also allows the user to inject faults in images, but it additionally provides a simple intuitive graphical interface as well as the ability to perform the injection retrospectively or in real-time.
    
    In the domain of Unmanned Aerial Vehicles (UAV), the authors in \cite{hsiao2021mavfi} present a ROS-based application the system is built as a ROS node and leverages the ROS communication protocol and Linux system to inject faults. As an illustrating example, the authors analyse the effect of corrupting the execution of modules related to the generation of the flight command and measure the impact on the quality of flight. 
    
    \subsubsection{Strengths} 
    It improves the reliability of the system. The faults injected can mirror real-world conditions. Demonstrating resilience can build confidence in the system.
    
    \subsubsection{Weaknesses}
    Designing and implementing fault and(or) noise injection scenarios can be complex. Injected faults might lead to scenarios that never occur in the real world. The injection process can be resource-expensive and time-consuming.

\subsection{MTA2. Exploit automation for test case generation, test case prioritization and selection, oracle and monitor generation}\label{sec:GMTC2}

    \subsubsection{Context (WHEN)} Automation of testing activities is getting increasing attention in the robotic domain, even in the case of field-based testing. Automation can be exploited for various activities, including test case generation~\cite{hutchison2018}, prioritization, selection, and oracle generation. The benefits brought by automation are various: it helps improving the efficiency, effectiveness, and reliability of the software testing processes, e.g. by increasing the test coverage and providing consistency and repeatability in the testing process. %For instance, in~\cite{hutchison2018}, the authors proposed an approach that automatically generates and runs tests to effectively find defects in real-world and industrial autonomous systems.
%    Test case design is fundamental when testing robots in the field. Field tests can be expensive, and slow. The choice of the test cases to be carried to runtime should be carefully defined. 
%    Applying automation to the test case generation, prioritization, selection and oracle generation in the testing of robotic systems is an appealing concept. 
    However, when applying automation in testing there are several challenges to be considered~\cite{afzal:2020}. First, it needs to deal with the environmental complexity and its high variability.  Second, specifying and/or generating an oracle that automatically distinguishes between correct and incorrect behaviours is not always obvious. Consequently, the test automation in field-based testing, is still limited and relies heavily on human contributions~\cite{bertolino:2021}. 
%    In spite of these challenges, adding automation can increase considerably the test coverage and provide consistency and repeatability in the testing process.
%    For instance, in~\cite{hutchison2018}, the authors proposed a system that can automatically generate and run tests to effectively find defects in real-world and industrial autonomy systems.
    \subsubsection{Reason (WHY)} 
    Automating testing activities can improve efficiency, as they can be run quickly and repeatedly without human intervention. This leads to quicker feedback on the quality of the software. Also, automation  is essential to enhance the efficiency, effectiveness and reliability of the software testing processes. Moreover, as the system grows and evolves, automated test suites can generally be extended easily to accommodate new features and changes.
    Indeed, there is an initial investment to be made in creating and maintaining the automation machinery. 
%    Furthermore, while there is an initial investment in creating and maintaining automated tests, it is essential to enhance the efficiency, effectiveness and reliability of the software testing processes.
    
    \subsubsection{Suggestion (WHAT)}
     The QA team should exploit automation tools for test case generation, test case selection and oracle generation, as well as other testing activities, to efficiently gain confidence in ROS-based systems in the field. For example, Mithra (pdf: https://afsafzal.github.io/materials/AfzalMithra.pdf) learns oracles from logs generated during the execution, it is motivated by a case from ArduPilot and tested in autonomous racing cars built on ROS. In addition, HAROS (git: git-afsantos/haros) promotes test case generation from properties using a tool called Hypothesis (git: HypothesisWorks/hypothesis). Finally, a technical report (pdf: https://www.cse.chalmers.se/$\sim$bergert/paper/2022-iros-roboticstesting.pdf) details how a company building mobile robots for disinfection uses equivalence partitioning for test case selection for the field.

    \subsubsection{Process (HOW)}
    % \subsubsection{Process (HOW)} \ric{The process should contain all the citations and exemplars from the exemplars section. If possible, ordered. The point of the process is actually to guide the testers into applying what is written in the suggestion. In this case, the question we want to answer is: ``How can the tester explore/use/exploit automation tools in the various stages of testing?''}
    To effectively implement test automation, one important step concerns the oracle specification, which is a mechanism or criteria to determine whether a test has passed or failed \cite{barr2014oracle}. A novel approach in automatic oracle generation based on telemetry data which is validated using a ROS-based system is proposed in~\cite{afzal2021mithra}. 
    % In~\cite{ferrando:2020}, the authors present a modular approach to oracle definition. \pat{is this in robotics? What they do more concretely? It would be nice to refer to ROS} 
    An important automation activity is the test case generation, with the aim of crafting tests cases to cover various functionalities, scenarios and edge cases of the system. For achieving this, a viable approach is to use Property Based Testing~\cite{santos2018property}, where test cases are automatically generated to target specific properties of the system. Another important automation activity concerns the test selection, which aims to select, in the search for efficiency, the relevant and representative scenarios to be tested. In this area, equivalence testing is a technique that allows us to reduce the amount of test cases used by dividing the generated cases in equivalence classes, as evidenced in ~\cite{ortega2022testing}, where the authors study ROS-based systems in the domain of service robotics. 
    
    \subsubsection{Exemplars}~\\
    {\bf Technology enablers:}  
    As a technology enabler, rostest\footnote{\url{http://wiki.ros.org/rostest}} is a ROS framework that allows us to do full integration testing across multiple nodes. In the task of test case generation in particular, one crucial component of the library is unit test. This module makes it possible to perform ROS node integration-level tests as well as code-level unit tests. In the case of ROS 2, the testing mechanism is ingrained in the structure of the packages, which makes the test development considerably easier. 

    {\bf Oracle specification:}  
    In the area of automated oracle generation, the authors of~\cite{afzal2021mithra}  present \textit{Mithra}, which is a novel and unsupervised oracle learning technique for Cyber-Physical Systems (CPS). The approach is applied to autonomous racing cars built for ROS.
    The oracle learning approach builds oracles by clustering telemetry logs represented by a novel formulation of multivariate time series (MTS) that effectively and concisely encodes correct CPS behaviour. 

    {\bf Test case generation:} 
    % property-based test case generation~
    Santos et al.~\cite{santos2018property} rely on property-based testing (PBT) to generate test cases driven by properties specified in the form of assertions.
    %As an illustrating approach to test case generation, in \cite{santos2018property}, the authors use Property-Based Testing (PBT), which is a technique in which the testing process is driven by the specification of generic properties that a system should satisfy.
    The tool \href{https://github.com/HypothesisWorks/hypothesis}{Hypothesis~\faicon{github}} receives a model of ROS configurations and generates customizeable property-based scripts for tests aimed at these configurations. It builds on top of configuration models extracted using HAROS, a static analysis framework for ROS applications.

    As another example, in the domain of mobile robots, the work in~\cite{hildebrandt2020feasible} presents an approach to automatically generate test cases in the form of stressful trajectories. In essence, the work integrates kinematic and dynamic physical models of the robot to generate valid trajectories. The test case generator incorporates a parameterizable scoring model to efficiently generate valid yet stressful trajectories for a broad range of ROS-based mobile robots. 
    
    {\bf Test case selection:} 
    As a test selection mechanism, one commonly used technique is Equivalent Partitioning. The objective of equivalence partitioning is to minimize test case explosion, i.e. reduce the high number of possible combinations of the properties that will be tested. 
    The idea behind Equivalence Partitioning is to group the test cases into equivalence classes according to how they handle valid or invalid data~\cite{ortega2022testing}. The authors report the experience of field testing in the domain of service robotics. In particular, the system under study was the Kelo AD disinfection robot whose software stack is based on ROS. To implement the equivalence testing, the criteria for defining the  classes included robot motion, person posture, existence of occlusions and obstacle positions. 

% \pat{check this, from ROSIN project ``Testing-Based Validation Infrastructure for ROS": \href{https://ec.europa.eu/research/participants/documents/downloadPublic?documentIds=080166e5d10078bc&appId=PPGMS}{rosin}}

% \pat{\href{http://wiki.ros.org/rostest}{rostest}. This can be also interesting: \href{http://wiki.ros.org/unittest\#ROS-Node-Level_Integration_Tests}{unittest}}

% \pat{automatic testing in ROS: \url{http://wiki.ros.org/Quality/Tutorials/UnitTesting}, and ROS2: \url{https://docs.ros.org/en/iron/Tutorials/Intermediate/Testing/Testing-Main.html}}

% \pat{ROBOFUZZ: \url{https://dl.acm.org/doi/abs/10.1145/3540250.3549164}, \url{https://github.com/sslab-gatech/RoboFuzz}}
    \subsubsection{Strengths} 
    Automation in testing activities can be executed repeatedly with low effort and cost. Moreover, it brings benefits in terms of efficiency, effectiveness, and reliability. 
    %It can cover a wide range of scenarios and increase the testing speed.
    \subsubsection{Weaknesses}
    There is a high initial investment of time and resources. There is also a maintenance overhead related to maintaining the automation machinery when the system evolves. 
    {\color{blue} Test generation may not scale for complex scenarios.}\footnote{Added after follow-up questionnaire on April 14th.}

\subsection{SE1. Use record-and-playback when performing exploratory field tests}\label{sec:SE1}

    \subsubsection{Context (WHEN)} %Field testing is slow and expensive. 
    In order to effectively select which test scenarios should be escalated to the field, the testing teams often perform exploratory field tests~\cite{bertolino:2021}.  %Exploratory field testing consists of field tests following agile-like development-test cycles. 
    Exploratory testing is an experience-based technique where the tester designs and executes tests based on prior knowledge, previous tests, curiosity, and other heuristics for common failures~\cite{reid2013software}.  %may help gain confidence in what test scenarios should escalate to the field. 
    For instance, exploratory field tests may be useful for identifying corner cases that could be missed during design~\cite{ortega2022testing}, or calibrating (e.g., tuning parameters~\cite{Caldas2020,zahn2019optimization}) the system under scrutiny before committing to the field test scenario. ROS practitioners typically use Record and Playback (aka record-and-replay) for testing, debugging and developing new algorithms~\cite{afzal:2020}. 
    %ROS-based systems are typically cyber-physical and are constructed over feedback loops.
    Record-and-playback is especially useful for performing exploratory tests of feedback loop systems since they provide lightweight means to record execution traces without preventing the testing team from freely exploring scenarios in the field.
    %replicate interactions of the closed loop~\cite{hutchison2018}. 
    In ROS, record-and-playback is a technique that consists of recording message exchange between ROS nodes and enabling the user to reproduce the set of recorded messages in a specific order. The nominal use of record-and-playback, however, does not necessarily consider information from the field, placing the assessment (i.e., testing, debugging, analysis) in jeopardy. 

    \subsubsection{Reason (WHY)} Escalating exploration scenarios to the field asks for lightweight means to recording data for scenario reproduction. 

    \subsubsection{Suggestion (WHAT)} %The quality assurance team should use record-and-playback in order to keep track of the explored field scenarios.
    When running exploratory field testing, the QA team should use record-and-playback in order to keep track of the explored field scenarios, simplify error analysis, find and reproduce corner cases, and help with parameter tuning. The standard tool for record-and-playback in ROS is rosbag (wiki: http://wiki.ros.org/rosbag) but there are a few tool derivations supporting effective record-and-playback. For example, Rerun.io (git: rerun-io/rerun) promotes a graphical interface with a focus on the visualization of bag data leveraging common datatypes used on perception algorithms. In addition, NuBots (git: NUbots/NUbots) uses a genetic algorithm for tuning parameters for the RoboCup over data collected in field explorations after data bags.

    \subsubsection{Process (HOW)}  Record-and-playback is well known by the ROS community. The ROS environment provides rosbag, a package that natively enables record-and-replay, which is frequently maintained and active. A few tools extend rosbags with addons to more expressive visualizations and data types (e.g., Rerun.io) or building on largely used behavior models (i.e., behavior trees) to replay robot behavior within mixed-reality scenarios~\cite{han2022mixed}. Moreover, record-and-replay for exploring field testing scenarios used for simplifying error analysis~\cite{beul:2017}, finding corner cases~\cite{ortega2022testing}, and parameter tuning~\cite{zahn2019optimization,Caldas2020}.

    \subsubsection{Exemplars}~\\
    \textbf{Technology-enabler:} The standard library for record-and-playback in ROS is \href{https://github.com/ros/ros_comm/tree/noetic-devel/tools/rosbag}{rosbag~\faicon{github}} (or \href{https://github.com/ros2/rosbag2}{rosbag2~\faicon{github}}).
    The rosbag package provides a means for recording exchanged messages in so-called bag files and reproducing the messages between components in release order. In addition, the package contains tools for analyzing, processing logs, and visualizing exchanged messages. 
    Recent research, builds on top of rosbag to encode more expressive tooling for applying records and reproducing for testing purposes, for instance using behavior trees to replay robot behavior in mixed reality~\cite{han2022mixed}.  
    \href{https://github.com/rerun-io/rerun}{Rerun.io~\faicon{github}} provides a general-purpose tool with focus on visualization of bag data which leverages common datatypes used in perception stack for robotics applications. Rerun enables URDF scene plotting, with 2d and 3d transformations, camera, odometry and tf transforms (e.g., rerun/ros\_node example~\href{https://github.com/rerun-io/rerun/blob/main/examples/python/ros_node/main.py}{\faicon{github}})\\
    {\bf Simplifying error analysis:} Beul M. et al.~\cite{beul:2017} extensively used bags to record the state of their unmanned aerial vehicle during field testing, keeping rosbag activated even in between experiments to avoid setting up overhead. Once the experiments are done, the authors filter and analyse the data using in-house tools including recording mission executions, editing traces and loading them for testing purposes. Finally, the authors claim that the toolset helped by simplifying the error analysis that was running over exploratory field scenarios (named experiments) where they logged user-defined missions in terms of ordered sets of 4D waypoints.\\
    {\bf Finding corner cases:} Ortega A. et al.~\cite{ortega2022testing} studied field testing experiences with an industrial-strength service robot (i.e., for hospital disinfection) transitioning from lab experiments to an operational environment. They conclude that the field testing strategies employed can be categorized into two phases, exploratory field testing and field endurance tests. Exploratory field testing helps find defects caused by variability in the environment, thus identifying corner cases~\cite{ortega2022testing}. However, replicating corner cases is challenging due to a lack of tooling to extract data from the field experiments. After all, the data collected from the fields must be (re-)useable, asking for tooling such as record-and-replay. \\
    \textbf{Parameter tuning:} Algorithms using multi-objective optimization for improving functionality~\cite{zahn2019optimization} or managing quality attributes (e.g., reliability) at runtime~\cite{Caldas2020} may benefit from recording data in exploration scenarios and playback for tuning parameters. Zahn b. et al.~\cite{zahn2019optimization} implements NUbots and uses a genetic algorithm (namely NSGA-II) to tune the parameters of a kicking strategy for a football robot player in the Robocup, for that, they rely on record-and-playback. \href{https://github.com/NUbots/NUbots}{NUbots~\faicon{github}}, however, instead of relying on standard ROS tooling to record-and-playback provide their own implementation. Similarly, Caldas et. al~\cite{Caldas2020} uses an implementation of their own to record whether a healthcare system (namely \href{https://github.com/lesunb/bsn}{BSN~\faicon{github}}~\cite{Gil2021}) presents faults at task-level execution, then playback the recorded data in a data mining pipeline (using also NSGA-II) to tuning the parameters of a software controller. 

    \subsubsection{Strengths} Record-and-playback is a good instrument to reduce the need for maintenance during quality assurance. It fosters also the repeatability of scenarios that would be rather lost when exploring field scenarios in an ad hoc way.
    
    \subsubsection{Weaknesses} Record-and-replay may not scale well~\cite{koo2019distributed}, can be the door for security exploits~\cite{jeong2017study}, and lacks means for fine-grained control of their recording thus the emergence and need for extensions to rosbag.

\subsection{SE2. No GUIs! Prioritize headless simulation}\label{sec:ETC2} 

    \subsubsection{Context (WHEN)} 
    Simulation is a great way to validate that a robot behaves as expected~\cite{afzal:2020}. It can also be used in hybrid approaches to combine real data from field with simulation engines, therefore making the testing more realistic~\cite{hildebrandt2021world}. Then, simulation can be useful as an isolation mechanism for testing, given that it can separate in-vivo testing from the production processes by reproducing the main process in a simulator based on information gather from the main execution by means of probes~\cite{bertolino:2021}. Furthermore, as mentioned in \cite{hutchison2018}, the QA team can use replay and subsystem testing to check the behaviour of certain components of the system without a full simulation by starting them up in isolation and replaying the logs. Running the simulators stripped of their Graphical User Interface (GUI), also referred to as headless simulation, allows QA teams to (i) scale up the testing of the robot behavior towards large-scale experimentation, (ii) reduce the resources consumption, and (iii) properly organize experiment with automatic generation of scenarios, operation environments where the robots should act, and/or automatic injection of noise or uncertainty. %In addition, headless simulation is useful as an isolation mechanism for testing, given that it can separate in-vivo testing from the production processes by reproducing the main process in a simulator based on information gather from the main execution by means of probes\cite{bertolino:2021}. 
    % \ric{what if we focus on offline field testing from \cite{bertolino:2021} to motivate this guideline?}

    \subsubsection{Reason (WHY)}
    Running the simulation headlessly allows one to avoid the overhead of rendering graphics and updating the GUI, as well as help in saving computational resources. Furthermore, headless simulation enables automation and make it feasible to integrate simulation with testing activities and incorporate it into continuous integration / continuous deployment (CI/CD) pipelines.

    \subsubsection{Suggestion (WHAT)}
    When it is possible to test or verify without human supervision, the QA team should prioritize headless simulation to avoid unnecessary overhead, enable large-scale experimentation, and facilitate integration with CI/CD pipelines. Example of tools supporting headless simulation are Gazebo (git: gazebosim/gz-sim), V-REP (wiki: http://wiki.ros.org/vrep\_ros\_bridge), ARGOS (web: https://www.argos-sim.info/), MORSE (https://morse-simulator.github.io/), and MVSim (git: MRPT/mvsim). As a complement, OpenDaVINCI (git: se-research/OpenDaVINCI) interfaces with ROS and has been widely used for testing autonomous driving systems.
    
    \subsubsection{Process (HOW)}
    To run a simulator in headless mode, the user typically needs to specify a particular command-line argument or configuration setting before initiating the simulation. Although, in most of these simulators, the visual interface and the simulation engine are tightly coupled \cite{estivill2018continuous}, many of them, including Gazebo, V-REP, ArGoS~\cite{Pinciroli:SI2012,pitonakova2018feature}, MORSE, MVSim, and OpenDaVinci~\cite{berger2016open} allow for this setting to be set.
    \subsubsection{Exemplars}~\\
    \textbf{Technology Enablers}: 
    Most of the widely used simulators in the domain of robotics have a way to specify the intention of running the simulation headless. In Gazebo, it is done by specifying an option either through the command line or in the launch file\footnote{\href{https://answers.gazebosim.org/}{https://answers.gazebosim.org/}}, although as stated in \cite{estivill2018continuous}, there is still some instability in the support of this feature. V-REP also allows a user to set a headless simulation by adding a special option in the execution of the program.\footnote{\href{http://www.forum.coppeliarobotics.com}{http://www.forum.coppeliarobotics.com}} Furthermore, the ARGOS simulator \cite{Pinciroli:SI2012}, created to support the simulation of large scales swarms of robots, efficiently supports a headless mode of operation; it has been proven to outperform Gazebo and V-Rep simulators when running headless in small scenes with up to 10 robots~\cite{pitonakova2018feature}.

    Other simulators that allow headless operations include \href{https://morse-simulator.github.io/}{MORSE~\faicon{github}}, although the feature has only been tested in Linux, and \href{https://github.com/MRPT/mvsim}{MVSim~\faicon{github}}, which is a lightweight simulator capable of running real-time scenarios for multiple vehicles.

    \textbf{Use cases}: 
    % \ric{I miss a section with examples on how can testers use headless simulation during system execution to testing and verification of ROS-based systems. I recall that there are some papers on this in our list of papers. Example: \cite{beul:2017,balakrishnan:2021,duan2021implementing,guerrero:2021,hartsell:2019,lewis:2022,liu:2017}. All of these are results from the literature review. They cite the word simulation. I am unsure if it is headless and can be used at runtime, but may turn out to be useful to explaining the concept here. We can look tomorrow into papers together.}
    The authors of~\cite{estivill2018continuous} propose a paradigm to incorporate validation via headless simulation into the continuous integration cycle. In addition to providing an illustrating use case of how to build and connect the different component of such a system, they provide a set of generic steps to be followed during the setup phase. 
    The authors of~\cite{berger2016open} develop a system in which they setup a virtual test environment targeting algorithms that will run in complex autonomous driving systems. As a result of this work, they build the open source environment OpenDaVinci, which includes libraries that enable the reuse of the algorithms to be tested in headless simulations as part of unit tests. They demonstrate how to use the framework in combination with the simulation environment to develop a self-parking algorithm~\href{https://github.com/se-research/OpenDaVINCI/tree/master/automotive/miniature/studies/example-boxparker}{\faicon{github}}.
    % \pat{\url{https://aws.amazon.com/blogs/robotics/build-headless-robotic-simulations-with-aws-batch/}}
    % \pat{check this: \url{https://answers.ros.org/question/154511/fast-headless-robot-simulator/}}

    % \pat{Microsoft: \url{https://learn.microsoft.com/en-us/previous-versions/microsoft-robotics/dd190946(v=msdn.10)}}
    % \url{https://answers.gazebosim.org//question/5387/gazebo-on-headless-simulation-server/}
%     \pat{Check this: ,
% % \url{https://robocomp.github.io/web/gsoc/2019/nikhil_bansal/post02},
% % \url{https://www.sciencedirect.com/science/article/pii/S2352711023001395},
%     \url{https://ceur-ws.org/Vol-2245/morse_paper_3.pdf}, Headless benchmark: \url{https://lenkaspace.net/downloads/Pitonakova_simulatorsComparison.pdf}
%     }

    \subsubsection{Strengths} 
    With headless simulation, the feedback is obtained faster, the simulations therefore can scale across multiple processors and cloud servers, and it makes possible to integrate the simulation into continuous integration pipelines.
    
    \subsubsection{Weaknesses}
    Debugging is more challenging without visual feedback as it is considerably more difficult to locate the issues or understand unusual behavior.

\subsection{AR1. Perform postmortem analysis to diagnose non-passing test cases}\label{sec:AR1} 

    \subsubsection{Context (WHEN)} The test case execution phase results in reports yielding a set of ran test cases paired with Boolean results attesting whether the cases passed or failed. Failing test cases, often, indicate the reason for failure by comparing the expected outcome with the actual outcome. However, that may not be enough to understand \textit{why did the robot fail} that test case, since such assertions do not comprehensively entail structural information about how the ROS-based system under test works. Such lack of information poses a risk to the usefulness of the executed tests. In order to provide fruitful information back to the development team, the testers should make the most out of the data by delving into a postmortem analysis for deriving explanations for the failed case~\cite{falcone:2021}.
    
    \subsubsection{Reason (WHY)} The postmortem analysis is essential for understanding the reasons behind the failure of test cases in ROS-based systems.
    
    \subsubsection{Suggestion (WHAT)} %In order to further understand false verdicts, the QA team should perform postmortem analysis and diagnose non-passing test cases.
    The QA team should perform postmortem analysis and diagnose of non-passing test cases to explain the failures to developers or refine the arguments and confidence in the robotic system. For example, ROS projects may use a combination of Nagios (web: https://www.nagios.org/) and ros/diagnostics for monitoring, collecting and aggregating runtime data to diagnose failures. Moreover, CARE (git: softsys4ai/care) may be used for semi-automatic diagnosis of launch file misconfigurations or may rely on approaches such as Rason (git: lsa-pucrs/rason/) for multi-robot diagnosis.
    
    \subsubsection{Process (HOW)}  Natively, ROS provides a diagnostics infra, the ros/diagnostics package\footnote{\href{http://wiki.ros.org/diagnostics}{http://wiki.ros.org/diagnostics}}, the package enables manual data aggregation and analysis\footnote{\href{http://wiki.ros.org/diagnostics/Tutorials/Analyzing_Diagnostic_Logs}{An official tutorial on analysis using the diagnostics package.}}. However, unveiling explanations for the test case failure requires better support. The testing team may rely on visualization techniques~\cite{roman2018overseer}, semi-automatic diagnostic generators~\cite{hossen2023care,kirchner2013rosha}, and deployment of extra infrastructure to support explanations with more data~\cite{morais2015distributed}.

    \subsubsection{Exemplars}~\\ 
    \textbf{Visualization:} Often, roboticists need to use their technical experience to identify points of failure and diagnose failed test cases. With that in mind, Roman F. et al.~\cite{roman2018overseer} propose Overseer, an architecture that unites Nagios (i.e., a general-purpose open-source monitoring tool\footnote{\href{https://www.nagios.org/}{https://www.nagios.org/}}) and ros/diagnostics (i.e., standard tooling for collecting and aggregating runtime data in ROS) as a key-enabler to visualization the runtime information and, in consequence, diagnostics. The overseer implements a monitoring server responsible for persisting data generated during the experiments in a database that can be later accessed by Nagios. \\
    \textbf{Semi-automated diagnosis:} Causal Robotics DEbugging (CARE)~\cite{hossen2023care}~\href{https://github.com/softsys4ai/care}{\faicon{github}} is a two-phase method for diagnosing configuration faults (aka misconfigurations) in ROS-based systems. The method proposes first a causal model learning step, then an inference over the learnt model step. The causal model is three-layered and defines causal relations between (i) software-level configurations or hardware-level options (e.g., sensors), (ii) a map from configuration options to how they influence the outcome performance, and (iii) performance goals. The authors employ Fast Causal Inference (FCI) to extract the causal model from data. Moreover, the authors present an algorithm for causal path discovery (by inference) which finds a locally optimal path between configuration (aka symptom) and performance goal. Following a similar idea of three layered causal models, Kirchner D. et al. implemented RoSHA~\cite{kirchner2013rosha} an architecture for self-healing robotic systems implemented in ROS. Their approach relies on monitoring, diagnosis, recovery management and execution. In order to implement the automatic diagnosis, RoSHA relies on the standard tool ros/diagnostics to collect runtime failure information (i.e., w.r.t. component dependencies, communication, and time relations between components) to identify why the robot fails. The collected information is regarded as symptoms, which are fed into a Bayesian network in order to compute the correlations between symptoms and root causes. Both techniques for diagnosis require structural constraints in the model to be feasible, asking for manual assistance to the diagnosis.\\ 
    \textbf{Multi-robot diagnosis:} Morais et al.~\cite{morais2015distributed}, promotes an approach for collaborative fault diagnosis using behavior trees in an agent programming language style, namely Rason~\href{https://github.com/lsa-pucrs/rason/}{ \faicon{github}} \cite{morais2015distributed}. The approach relies on deploying an extra robot to assist a faulty robot in diagnosing a fault. Whenever the faulty robot identifies a verdict of fault in their behavior, the extra robot is activated to examine and provide extra information to disambiguate the diagnostic. For example, when a faulty robot does not identify that there is a mechanical issue with their wheel and \textit{cannot reach their destination (verdict)}, the extra robot examines their wheel with a camera and identifies an issue. Following the analogy, the testing team may consider the deployment of extra robots to collect more information to assist with the diagnostics. Swarmbug~\cite{jung2021swarmbug} is an approach for debugging configuration bugs in swarm robotics. It abstracts the impacts of environment configurations (e.g., obstacles) on the drones in a swarm and automatically generates, validates, and ranks fixes for configuration bugs. 

    \subsubsection{Strengths} A benefit of postmortem analyses in comparison to on-the-fly analyses is that the former, with full traces, presents better potential to improve the explanation precision~\cite{falcone:2021}.

    \subsubsection{Weaknesses} Diagnosis may require manual effort and domain knowledge to be effective, diagnosing without domain experience may lead to false positives.

\subsection{AR2. Use reliable tooling in order to manage field data}\label{sec:AR2} 

    \subsubsection{Context (WHEN)} Maintaining the field resources is a fundamental step for the repeatability and reliability of field tests~\cite{bertolino:2021}. The field data is useful for generating field test cases and postmortem analyses. Yet, the data generated before, during and after testing must be kept and managed. Field data management often includes storing new data, annotating data, and generating reports. Such activities may turn intractable as the number of trials grows along with the complexity of the stored data (i.e., in perception systems, or learning-enabled systems). Manually managing such data is error-prone and sometimes unfeasible. 
            
    \subsubsection{Reason (WHY)} Field testing is expensive and relying on ad hoc solutions to storing data may result in corrupted or incomplete field data. Unreliable tooling may be a source of flaky tests or skewed conclusions about the system (i.e., false-positive results). 

    \subsubsection{Suggestion (WHAT)} The QA team should use reliable tools for field data management to avoid problems with corrupted, unreliable, and/or incomplete data. For example, the warehouse\_ros package offers both MongoDB (git: ros-planning/warehouse\_ros\_mongo) and SQLite (git: ros-planning/warehouse\_ros\_sqlite) database backend for recording states, scenes, and messages. In addition, the Field Test Tool (git: fkie/field\_test\_tool) uses the PostgreSQL database manager extended with PostGIS for geolocalization.
        
    \subsubsection{Process (HOW)} Testers may use local workspace standard tooling aided by git-based versioning~\cite{ortega2022testing} or structured database~\cite{roman2018overseer,tampier2022field}, and file-server~\cite{hartsell:2019}, for field data management. On the one hand, using local workspace tooling is intuitive since tutorials in ROS traditionally rely on them, and most developers are used to the workspace management tools. On the other hand, structured approaches using database management tools may render easier querying and means to automatic report generation. When it comes to database integration for persisting long-term data, Malavolta et. al suggest using a dedicated node to interface the application and the database system in order to mitigate performance issues~\cite{malavolta2021mining}.
    
    \subsubsection{Exemplars}~\\ 
    \textbf{Local workspace with git support.}
    Ortega A. et al. reports about the maintenance of test documents and artifacts for testing in the field~\cite{ortega2022testing}. The documents contain the specification of test procedures, reports, rosbag files, incident reports and cases in which people are detected. Test reporting is done on an in-house tool called Technology Readiness Level Test Report Library (TRL) and the reports are stored in a git repository where test incidents issues. TRL is based on the standard tooling for local workspace management in ROS, namely wstool~\footnote{\href{http://wiki.ros.org/wstool}{http://wiki.ros.org/wstool}}. \\
    \textbf{Database and File-server.}
     The warehouse\_ros package provides MongoDB (\href{https://github.com/ros-planning/warehouse_ros_mongo}{WRM \faicon{github}}) and SQLite (\href{https://github.com/ros-planning/warehouse_ros_sqlite}{WRS \faicon{github}}) database backend for persistently recording states, scenes and messages, working in conjunction with RViz and the MotionPlanning plugin. The Field Test Tool (\href{https://github.com/fkie/field_test_tool}{FTT \faicon{github}}) provides support for logging, annotating, and automatically generating reports of field trials for autonomous ground vehicles~\cite{tampier2022field}. The tool relies on a database to store field data, which is later accessed for automatic report generation. The authors use PostgreSQL database manager extended with PostGIS for geolocalization. The data is stored in the database through an interface ROS node which collects field data (Operation mode, GNSS positioning, local positioning, a map of the environment, and possibly images from a camera) from selected topics. Data collection is started and stopped in a web server that interfaces with the tester. The web interface can also be used to add annotations to collected field data. In addition to FTT, the Overseer architecture~\cite{roman2018overseer} enables the persistence of field data in a MySQL database, which can be further accessed by the monitoring system Nagios. On another stance, Hartsell et al.~\cite{hartsell:2019} studies ROS-based systems with learned-enabled components. Often, testing such systems is prone to large dataset maintenance, which can be a problem in the field. The author's approach uses a mix of file servers for storing the data and a database for storing metadata. The file server relies on SSH File Transfer Protocol (SFTP) to store all generated data, resulting from the execution of a job (aka trial),  results and notes from the experiments. The metadata is persisted in a version-controlled database for quick retrieval. As far as we are concerned, even though Hartsell's approach should work for field testing it was only validated in simulation testing~\cite{hartsell:2019}.  % \cite{hartsell:2019} approach is talking about simulation testing, read 4.5 Experiment Gyms. Although they mention real-world experiments, it is left to the future work. I could not find the extension with the real-world experiments.

     % Should we also include this paper? 
     % Fiannaca, Alexander J., and Justin Huang. "Benchmarking of relational and nosql databases to determine constraints for querying robot execution logs." Computer Science & Engineering, University of Washington, USA (2015): 1-8. 

    \subsubsection{Strengths} Tool support for persisting field data helps with data reliability since it is less likely that data will be lost or will be corrupted. In addition, this guideline enables traceability of trial execution with possible failure or fault.
    
    \subsubsection{Weaknesses} Using database systems to log long-term data may pose a threat to the performance of the testing apparatus.
